# Supplementary material for: Incremental Learning in Semantic Segmentation from Image Labels
Source: arXiv:2112.01882 source file (2022-03-31)
Supplement: Supplementary file 1 [file supplementary.tex]

\section{Additional Implementation Details}
This section contains pseudo-code (Alg. \ref{pc:pseudo_code}) to help clarify the overall training procedure as well as further implementation details on the localizer training included in the \wilson\ framework.
We recall that the localizer, denoted as $g$, takes as input the features coming from the segmentation encoder $e$ to predict a score for all classes (background, old and new ones) \ie $z = g(e(x)) \in \real^{|\set{Y}^t| \times H \times W}$, where $\set{Y}^t$ is the set of classes seen (new and old) at the incremental step $t$.
In the main paper, we described two loss functions (the classification loss $\ell_{CLS}$ and the localization prior $\ell_{LOC}$) that we used to train the localizer. 
However, for the sake of space, we left to the supplementary material two additional losses.

\myparagraph{Pixel-wise refinement of the localizer output.}
Following \cite{araslanov2020single}, we introduced a self-supervised segmentation loss on the localizer output. This loss aims to force classification scores to be locally consistent, \ie near pixels with similar appearance should be assigned the same classification score.
First, we apply a refinement process on the classification output based on the pixel-level image similarity.
Then, we force the classification scores to be similar to the refined version by using a pixel-level segmentation loss only on the localizer without directly affecting the segmentation output.

To refine the classification scores, similarly to \cite{araslanov2020single}, we employ the \textit{Pixel Adaptive Mask Refinement} (PAMR). 
PAMR is a parameter-free module that iteratively refines the score of each pixel.
Starting from the normalized classification score $m  = \psi(z)$, PAMR refines it by considering the neighbour pixels $N(i)$.
We initialize $m^{ref,{0}} = m$ and, at the $t^{th}$ iteration the refined mask $m^{ref,t}$ is computed as:
\begin{equation}
     m^{ref,{t}}_i = \sum_{n\in N(i)} \alpha_{i, n} \cdot m^{ref,{t-1}}(n),
\end{equation}
where the pixel-level level affinity $\alpha_{i,n}$ is a value that measures the similarity among two pixels which is computed using a kernel function $k$ on the pixel intensities, so that:
\begin{equation}
    \alpha_{i, n} = \frac{e^{k(i,n)}}{\sum_{l \in N(i)} e^{k(i,l)}},
\end{equation}
where we followed the same definition of the kernel function $k$ defined in \cite{araslanov2020single} that considers the average similarity in pixel intensity on the RGB channels.
As suggested in \cite{araslanov2020single}, we used $3 \times 3$ neighborhood with different dilation rates, that we set to $\{1, 2, 4, 8, 12\}$, and we stopped after 10 iterations. Please refer to \cite{araslanov2020single} for additional details.

The refined classification scores are then converted to a pseudo ground-truth mask to compute the self-supervised segmentation loss. We ignored clashing pixels and we selected only pixels with a confidence higher than 60\% of the maximum value (greater than 70\% for the background class).
The localizer is then trained by optimizing a weighted cross-entropy loss:

\begin{equation}
    \ell_{SSS} = - \sum_{i \in I} \sum_{c \in \set Y^t} w_c \log m_{c,i} 
\end{equation}
with $w_c = \frac{|I| - M_c}{1+|I|}$ and $M_c = \sum_{i \in I} m^{ref}_{c,i}$, indicating with $_{c,i}$ the score of class $c$ at pixel $i$. 

\myparagraph{Encoder feature distillation loss.}  
Since the losses applied on the localizer are backpropagated on the segmentation encoder, it is possible that they will cause a shift in encoder representation, impacting negatively the segmentation performance. 

We use an additional \textit{feature distillation loss} to prevent the encoder's representation from shifting towards new classes and forgetting old ones.
In particular, we used a \textit{mean-squared error} function between the features extracted by the current encoder $e^t$, and the ones extracted at previous step $e^{t-1}$.
Formally, given an image $x$, the loss is computed as:
\begin{equation}
    \ell_{ENC} = \frac{1}{|I|} \sum_{i\in I} (e^t(x)_i - e^{t-1}(x)_i )^2,
\end{equation}
where $I$ is the set of pixels in the image and the suffix indicates the value at pixel $i$.

\myparagraph{Overall training procedure.} 
To sum up, the localizer has been trained, for the first 5 epochs, to minimize the following loss function:
\begin{equation}
    \ell_{TOT_{B5}} = \lambda_1 \ell_{CLS} + \lambda_2 \ell_{LOC} + \lambda_3 \ell_{ENC},
\end{equation}
where $\lambda_1$, $\lambda_2$, $\lambda_3$ are all set to $1$.

After the fifth epoch, we introduce the self-supervised segmentation loss, as in \cite{araslanov2020single}:
\begin{equation}
    \ell_{TOT_{A5}} = \lambda_1 \ell_{CLS} + \lambda_2 \ell_{LOC} + \lambda_3 \ell_{ENC} + \lambda_4 \ell_{SSS},
\end{equation}
with $\lambda_4=1$.

\myparagraph{Code.} 
The code to replicate \wilson\ has been attached to the supplementary material. The code provides the scripts to replicate \wilson\ and the baselines for all the settings. For the offline weakly-supervised methods, we refer to the official implementations\footnote{https://github.com/YudeWang/SEAM}~\footnote{https://github.com/halbielee/EPS}~\footnote{https://github.com/visinf/1-stage-wseg} to generate the pseudo-labels.

\begin{algorithm}[]
\SetAlgoLined
\SetKwBlock{Localizer}{Train the \textit{localizer} $g$}{end}
\SetKwBlock{Segmentation}{Train the segmentation model $f_\theta^{t}$}{end}

\textbf{Initialize:} 
    \\Model $f_\theta^{t-1}$ pre-trained on a densely-annotated dataset with label set $\mathcal{C}^{t-1}$\;
    Model $f_\theta^{t}$ with segmentation encoder $e$\;
    \textit{Localizer} $g$\;
\textbf{Input:} 
    $\mathcal{X}$, composed by set of pixels $\mathcal{I}$ with constant cardinality $N$, with image-level annotations $y$ for novel classes $\mathcal{C}^t$\;
\textbf{Output:}
    $y=\{\text{argmax}_{c\in \mathcal{Y}^t} p_i^c\}^N_{i=1}$, $p_i^c$ the model prediction of pixel $i$ for class $c$ and $\mathcal{Y}^t$ the set of seen classes\;
 
\While{epoch in max\_epochs}{
    \For{(x,y) in $\mathcal{X}$}{
        \Localizer{
            Compute score for all classes, as $z=g(e(x))$\;
            Compute output from previous model, as $\omega = \sigma(f_\theta^{t-1}(x))$, with $\sigma(\cdot)$ as the sigmoid function\;
            Aggregate pixel-level classification scores $z$ in $\hat{y}$ as the sum of \textit{normalized Global Weighted Pooling} (Eq. 1) and \textit{focal penalty} (Eq. 2)\;
            Train $g$ on $\mathcal{C}^t$ with multi-label soft-margin loss $l_{CLS}(\hat{y}, y)$ (Eq. 3)\; 
            Train $g$ with localization prior loss $l_{LOC}(z, \omega)$ (Eq. 4)\;
            \If{$epoch \ge 5$}{
                Train $g$ with self-supervised loss $l_{SSS}$ (Eq. A3)\;
            }
        }
        Train $e$ with encoder feature distillation loss $l_{ENC}$ (Eq. A4)\;
        \If{$epoch \ge 5$}{
            \Segmentation{
                Compute hard pseudo-labels $q_i^{\text{Hard,c}}$ from $g$ (Eq. 5)\; 
                Smooth $q_i^{\text{Hard,c}}$ in $q^c$ (Eq. 6)\;
                Compute pixel-level supervision label $\hat{q}$ from $q^c$ and $f_\theta^{t-1}(x)$ (Eq. 7)\;
                Train $f_\theta$ with multi-label soft-margin loss $l_{SEG}(f_\theta^{t}(x), \hat{q})$ (Eq. 8)\;
            }
        }
    }
}
\caption{Training WILSON}
\label{pc:pseudo_code}
\end{algorithm}

\section{Detailed results}
\subsection{Dataset class splits}
We provide an extensive evaluation of \wilson\ on the two standard benchmarks Pascal VOC 2012~\cite{Everingham2009ThePV} and COCO~\cite{lin2014microsoft}. 
Following previous work, we used two data settings on Pascal VOC: 15-5 and 10-10. To split the dataset, we follow the standard practice, and we divide them according to the alphabetic order.
\cref{tab:voc-split-15-5} and \cref{tab:voc-split-10-10} report the classes for the 15-5 and 10-10 settings, respectively.
For the COCO dataset, we split the classes according to their presence in the Pascal VOC dataset. In particular, classes in the Pascal VOC dataset are in the incremental step, while the others are in the base one. The split is reported in \cref{tab:coco-split}.

\subsection{Class-by-class results}
In this section, we report per class results on all the settings considered in the main paper. We considered the offline weakly supervised methods (WSSS) as baselines. At the same time, we could not report values for the incremental learning methods since these are not available in the considered published works.

\myparagraph{Single step addition of five classes (15-5).}
In \cref{tab:voc-15-5-d} and \cref{tab:voc-15-5-o} are reported the results for the disjoint and overlapped settings, respectively. From the tables, we can see that \wilson\ outperforms all the WSSS baselines on most of the classes. In particular, considering the disjoint setting, it obtains better results on 11 out of 15 old classes and 4 out of 5 novel ones. On the overlapped, \wilson\ obtains even better results, being best on 12 out of 15 old classes and all the new ones.
Moreover, in comparison with the joint training with pixel-level supervision, it achieves close results and, surprisingly, even superior on some old classes (\eg, \textit{bike, boat, bottle, chair, d.table, dog, person}). Differently, on the new classes, we still note a considerable performance gap, especially on classes with highly variable shapes, such as \textit{plant}.

\myparagraph{Single step addition of five classes (10-10).}
\cref{tab:voc-10-10-d} and \cref{tab:voc-10-10-o} report the results for the disjoint and overlapped settings. In this more challenging setting, the performance gap between \wilson\ and the WSSS baselines is reduced, but \wilson\ still obtains better results on the majority of the classes.
In particular, \wilson\ outperforms the baselines on 2 and 3 out of 10 old classes in the disjoint and overlapped scenario, respectively, and 
on 4 out of 10 new classes in both scenarios.
The difficulty of the setting is also confirmed by the comparison with the Joint training baseline. In particular, in the disjoint setting, \wilson\ achieves 10.6\% less mIoU on old classes and 19.7\% on the new ones, while in the overlapped setting, the performance improves on the old classes (-4.6\% mIoU) but decreases on the new ones (-16.9\%).

\begin{table}[t]
    \centering
    \begin{tabular}{c|p{5cm}}
         \textbf{step}  &  \textbf{classes} \\ \hline
         0  &  aeroplane, bicycle, bird, boat, bottle, bus, car, cat, chair, cow, table, dog, horse, motorbike, person \\  \hline
         1  &  plant, sheep, sofa, train, tv-monitor \\
    \end{tabular}
    \caption{Pascal VOC 15-5 class split.} \label{tab:voc-split-15-5}

\end{table}

\begin{table}[t]
    \centering
    \begin{tabular}{c|p{5cm}}
         \textbf{step}  &  \textbf{classes} \\ \hline
         0  &  aeroplane, bicycle, bird, boat, bottle, bus, car, cat, chair, cow \\  \hline
         1  &  table, dog, horse, motorbike, person, plant, sheep, sofa, train, tv-monitor \\
    \end{tabular}
    \caption{Pascal VOC 10-10 class split.} \label{tab:voc-split-10-10}

\end{table}

\begin{table}[t]
    \centering
    \begin{tabular}{c|p{6.5cm}}
         \textbf{step}  &  \textbf{classes} \\ \hline
         0  &  truck, traffic light, fire hydrant, stop sign, parking meter, bench, elephant, bear, zebra, giraffe, backpack, umbrella, handbag, tie, suitcase, frisbee, skis, snowboard, sports ball, kite, baseball bat, baseball glove, skateboard, surfboard, tennis racket, wine glass, cup, fork, knife, spoon, bowl, banana, apple, sandwich, orange, broccoli, carrot, hot dog, pizza, donut, cake,  bed,  toilet, laptop, mouse, remote, keyboard, cell phone, microwave, oven, toaster, sink, refrigerator, book, clock, vase, scissors, teddy bear, hair drier, toothbrush \\  \hline
         1 & person, bicycle, car, motorcycle, airplane, bus, train, boat, bird, cat, dog, horse, sheep, cow, bottle, chair, couch, potted plant, dining table, tv
    \end{tabular}
    \caption{COCO class split.} \label{tab:coco-split}
\end{table}

\myparagraph{COCO-to-VOC.}
COCO-to-VOC is the most challenging scenario proposed in the paper. Not only the classes to learn are more, but they also come from different datasets, 
\ie COCO on the base step and Pascal VOC on the incremental one.
We report the results on the incremental classes on VOC on \cref{tab:coco2voc-voc}. From the results, we see that \wilson\ obtains the best results, outperforming SS (the second best) by 1.5\% mIoU. Moreover, it achieves better results than the WSSS baselines on 11 out of 20 classes.
The results on the COCO dataset are reported in \cref{tab:coco2voc-coco}. We note that the most challenging classes are small objects that often appear with the person class, such as \textit{skii, handbag, baseball bat, skateboard, toaster, hair-drier}. The low performances can be explained considering that, at step $0$, we removed from COCO all the images containing at least a pixel from a class of VOC, including \textit{person}, significantly reducing the number of samples occurring often with it (\eg, \textit{skateboard, skii}) and compromising their performances.

\begin{table*}[t]

\begin{adjustbox}{width=1.0\textwidth}
\setlength{\tabcolsep}{3pt} 
\begin{tabular}{lc|cccccccccccccccc|ccccc|ccc}
\textbf{Method} & \textbf{Sup} & \textbf{bkg} & \textbf{aplane} & \textbf{bike} & \textbf{bird} & \textbf{boat} & \textbf{bott} & \textbf{bus} & \textbf{car} & \textbf{cat} & \textbf{chair} & \textbf{cow} & \textbf{d.table} & \textbf{dog} & \textbf{horse} & \textbf{mbike} & \textbf{person} & \textbf{plant} & \textbf{sheep} & \textbf{sofa} & \textbf{train} & \textbf{tv} & \textbf{Old} & \textbf{New} & \textbf{All} \\ \hline
Joint & Pixel & 92.5 & 89.9 & 39.2 & 87.6 & 65.2 & 77.3 & 91.1 & 88.5 & 92.9 & 34.8 & 84.0 & 53.7 & 88.9 & 85.0 & 85.1 & 84.9 & 60.0 & 79.7 & 47.0 & 82.2 & 73.5 & 76.5 & 68.5 & 75.4 \\ \hline
CAM                           & Image & 77.6&	74.9&	38.5&	73.5&	60.0&	72.4&	81.6&	86.7&	89.7&	32.4&	42.0&	56.0&	85.5&	77.8&	84.3&	84.6&	20.7&	15.9&	27.9&	32.7&	33.2&		69.3&	26.1&	59.4 \\
SEAM \cite{wang2020self}      & Image & 86.3&	79.6&	39.5&	81.3&	54.0&	66.0&	81.3&	85.2&	88.8&	34.2&	64.8&	56.2&	87.6&	80.2&	82.5&	84.5&	17.7&	36.6&	29.9&	45.2&	35.9&		71.0&	33.1&	62.7 \\
SS \cite{araslanov2020single} & Image & 86.4&	77.2&	38.7&	83.2&	62.0&	75.9&	76.5&	88.3&	89.1&	33.3&	63.1&	57.9&	84.0&	80.9&	79.9&	84.2&	18.6&	22.4&	20.3&	26.8&	41.9&		71.6&	26.0&	61.5 \\
EPS \cite{lee2021railroad}    & Image & 90.2&	83.9&	40.8&	84.9&	63.9&	75.7&	83.6&	86.9&	89.8&	34.0&	52.3&	56.4&	87.6&	82.6&	80.1&	83.9&	20.1&	43.9&	23.8&	64.8&	39.8&		72.4&	38.5&	65.2 \\
WILSON (Ours)                 & Image & 90.5&	88.8&	40.9&	86.4&	69.4&	77.9&	82.9&	88.0&	92.3&	35.4&	51.3&	56.2&	88.3&	83.9&	77.2&	85.1&	30.3&	47.5&	39.2&	54.6&	47.5&		\textbf{73.6}&	\textbf{43.8}&	\textbf{67.3} \\
\end{tabular}
\end{adjustbox}
\caption{Per class results on the Pascal VOC 15-5 Disjoint setting, expressed in mIoU. Best Image-supervised method in bold.} \label{tab:voc-15-5-d}
\end{table*}

\begin{table*}[t]

\begin{adjustbox}{width=1.0\textwidth}
\setlength{\tabcolsep}{3pt} 
\begin{tabular}{lc|cccccccccccccccc|ccccc|ccc}
\textbf{Method} & \textbf{Sup} & \textbf{bkg} & \textbf{plane} & \textbf{bike} & \textbf{bird} & \textbf{boat} & \textbf{bottle} & \textbf{bus} & \textbf{car} & \textbf{cat} & \textbf{chair} & \textbf{cow} & \textbf{d.table} & \textbf{dog} & \textbf{horse} & \textbf{m.bike} & \textbf{person} & \textbf{plant} & \textbf{sheep} & \textbf{sofa} & \textbf{train} & \textbf{tv} & \textbf{Old} & \textbf{New} & \textbf{All} \\ \hline
Joint & Pixel & 92.5 & 89.9 & 39.2 & 87.6 & 65.2 & 77.3 & 91.1 & 88.5 & 92.9 & 34.8 & 84.0 & 53.7 & 88.9 & 85.0 & 85.1 & 84.9 & 60.0 & 79.7 & 47.0 & 82.2 & 73.5 & 76.5 & 68.5 & 75.4 \\ \hline
CAM                           & Image & 77.0&	75.2&	38.3&	77.3&	60.5&	74.9&	71.3&	85.3&	88.4&	35.4&	54.8&	53.9&	86.5&	80.7&	81.2&	84.3&	16.6&	15.1&	28.3&	35.2&	33.0&		69.9&	25.6&	59.7 \\
SEAM \cite{wang2020self}      & Image & 85.3&	77.5&	39.6&	78.9&	53.9&	61.2&	58.7&	83.4&	87.8&	36.3&	69.6&	49.7&	86.3&	81.0&	76.9&	84.1&	13.0&	38.1&	29.8&	41.6&	36.2&		68.3&	31.8&	60.4 \\
SS \cite{araslanov2020single} & Image & 84.9&	78.7&	38.0&	82.2&	61.7&	74.9&	79.3&	85.4&	88.0&	40.1&	70.4&	56.9&	82.4&	81.7&	78.5&	84.3&	13.4&	27.4&	26.0&	32.7&	38.0&		72.2&	27.5&	62.1 \\
EPS \cite{lee2021railroad}    & Image & 89.6&	81.7&	39.4&	81.8&	63.6&	73.9&	53.2&	84.6&	88.1&	38.9&	53.1&	57.1&	86.8&	80.9&	74.0&	83.7&	16.4&	39.9&	27.8&	51.9&	36.7&		69.4&	34.5&	62.1 \\
WILSON (Ours)                 & Image & 89.5&	88.6&	41.2&	84.9&	68.7&	79.0&	83.9&	88.5&	91.7&	39.3&	55.7&	58.3&	89.0&	85.7&	73.3&	85.8&	26.5&	48.6&	36.6&	55.7&	40.9&		\textbf{74.2}&	\textbf{41.7}&	\textbf{67.2} \\
\end{tabular}
\end{adjustbox}
\caption{Per class results on the Pascal VOC 15-5 Overlapped setting, expressed in mIoU. Best Image-supervised method in bold.} \label{tab:voc-15-5-o}
\end{table*}

\begin{table*}[t]

\begin{adjustbox}{width=1.0\textwidth}
\setlength{\tabcolsep}{3pt} 
\begin{tabular}{lc|ccccccccccc|cccccccccc|ccc}
\textbf{Method} & \textbf{Sup} & \textbf{bkg} & \textbf{aplane} & \textbf{bike} & \textbf{bird} & \textbf{boat} & \textbf{bott} & \textbf{bus} & \textbf{car} & \textbf{cat} & \textbf{chair} & \textbf{cow} & \textbf{d.table} & \textbf{dog} & \textbf{horse} & \textbf{mbike} & \textbf{person} & \textbf{plant} & \textbf{sheep} & \textbf{sofa} & \textbf{train} & \textbf{tv} & \textbf{Old} & \textbf{New} & \textbf{All} \\
\hline 
Joint & Pixel & 92.5 & 89.9 & 39.2 & 87.6 & 65.2 & 77.3 & 91.1 & 88.5 & 92.9 & 34.8 & 84.0 & 53.7 & 88.9 & 85.0 & 85.1 & 84.9 & 60.0 & 79.7 & 47.0 & 82.2 & 73.5 & 75.1 & 74.0 & 75.4 \\
\hline 
CAM                           & Image & 78.5&	87.9&	35.6&	81.6&	62.3&	77.9&	76.6&	78.1&	73.1&	24.5&	56.1&	38.1&	41.9&	28.9&	50.2&	47.5&	37.6&	40.0&	34.1&	49.0&	45.2&		\textbf{65.4}&	41.3&	54.5\\
SEAM \cite{wang2020self}      & Image & 87.4&	88.8&	35.7&	84.4&	63.5&	77.2&	71.4&	66.6&	76.4&	27.6&	59.3&	42.1&	65.2&	45.6&	64.3&	59.3&	37.9&	67.9&	44.5&	56.1&	52.5&		65.1&	53.5&	60.7 \\
SS \cite{araslanov2020single} & Image & 81.2&	81.5&	25.3&	85.4&	64.5&	80.5&	78.0&	68.4&	60.1&	25.4&	38.4&	14.8&	17.2&	6.4&	26.1&	24.4&	29.7&	33.8&	21.1&	38.5&	45.5&		60.8&	25.7&	45.1 \\
EPS \cite{lee2021railroad}    & Image & 89.1&	79.2&	35.3&	85.2&	66.8&	80.2&	61.1&	70.6&	77.4&	26.0&	60.3&	38.1&	64.8&	51.1&	68.7&	66.8&	43.4&	50.8&	39.4&	73.8&	44.5&		64.2&	54.1&	60.6\\  
WILSON (Ours)                 & Image & 89.7&	78.8&	33.1&	87.7&	57.8&	80.9&	75.5&	71.3&	75.7&	28.7&	55.0&	27.7&	66.8&	43.3&	64.3&	59.5&	45.9&	63.2&	37.6&	74.3&	60.4&		64.5&	\textbf{54.3}&	\textbf{60.8}    
\end{tabular}
\end{adjustbox}
\caption{Per class results on the Pascal VOC 10-10 Disjoint setting, expressed in mIoU. Best Image-supervised method in bold.} \label{tab:voc-10-10-d}
\end{table*}

\begin{table*}[t]

\begin{adjustbox}{width=1.0\textwidth}
\setlength{\tabcolsep}{3pt} 
\begin{tabular}{lc|ccccccccccc|cccccccccc|ccc}
\textbf{Method} & \textbf{Sup} & \textbf{bkg} & \textbf{aplane} & \textbf{bike} & \textbf{bird} & \textbf{boat} & \textbf{bott} & \textbf{bus} & \textbf{car} & \textbf{cat} & \textbf{chair} & \textbf{cow} & \textbf{d.table} & \textbf{dog} & \textbf{horse} & \textbf{mbike} & \textbf{person} & \textbf{plant} & \textbf{sheep} & \textbf{sofa} & \textbf{train} & \textbf{tv} & \textbf{Old} & \textbf{New} & \textbf{All} \\
\hline 
Joint & Pixel & 92.5 & 89.9 & 39.2 & 87.6 & 65.2 & 77.3 & 91.1 & 88.5 & 92.9 & 34.8 & 84.0 & 53.7 & 88.9 & 85.0 & 85.1 & 84.9 & 60.0 & 79.7 & 47.0 & 82.2 & 73.5 & 75.1 & 74.0 & 75.4 \\
\hline
CAM                           & Image &78.4&	85.9&	38.7&	82.9&	68.4&	78.9&	82.7&	85.6&	83.0&	34.2&	67.5&	39.0&	51.1&	40.5&	53.7&	48.0&	39.1&	39.0&	37.1&	50.1&	44.5&		\textbf{70.8}&	44.2&	58.5 \\
SEAM \cite{wang2020self}      & Image &87.1&	84.2&	38.5&	84.4&	63.3&	77.2&	71.7&	69.6&	83.1&	33.7&	69.8&	44.5&	73.8&	60.5&	67.3&	59.2&	38.0&	65.1&	41.3&	54.9&	49.3&		67.5&	55.4&	62.7 \\
SS \cite{araslanov2020single} & Image &79.1&	85.8&	38.3&	84.1&	67.1&	79.4&	84.5&	84.8&	78.8&	34.0&	59.1&	17.4&	40.6&	31.9&	40.5&	23.6&	29.9&	37.9&	24.0&	38.4&	44.1&		69.6&	32.8&	52.5 \\
EPS \cite{lee2021railroad}    & Image &88.9&	87.3&	37.7&	84.4&	68.7&	77.6&	66.0&	75.5&	84.8&	35.8&	72.8&	38.9&	76.2&	65.5&	73.7&	66.7&	42.4&	50.8&	38.9&	76.0&	41.9&		69.0&	{57.0}&	64.3 \\
WILSON (Ours)                 & Image &89.1&	83.6&	38.1&	86.5&	62.8&	79.6&	79.3&	83.7&	85.4&	33.0&	72.3&	29.0&	77.8&	64.5&	73.9&	59.8&	40.9&	67.9&	37.5&	57.0&	62.3&		70.4&	\textbf{57.1}&	\textbf{65.0} \\

\end{tabular}
\end{adjustbox}
\caption{Per class results on the Pascal VOC 10-10 Overlapped setting, expressed in mIoU. Best Image-supervised method in bold.} \label{tab:voc-10-10-o}
\end{table*}

\begin{table*}[t]

\begin{adjustbox}{width=1.0\textwidth}
\setlength{\tabcolsep}{3pt} 
\begin{tabular}{lc|ccccccccccccccccccccc|c}
{\textbf{Method}} & \textbf{Sup} & {\textbf{bkg}} & {\textbf{person}} & {\textbf{bike}} & {\textbf{car}} & {\textbf{mbike}} & {\textbf{aplane}} & {\textbf{bus}} & {\textbf{train}} & {\textbf{boat}} & {\textbf{bird}} & {\textbf{cat}} & {\textbf{dog}} & {\textbf{horse}} & {\textbf{sheep}} & {\textbf{cow}} & {\textbf{bott}} & {\textbf{chair}} & {\textbf{sofa}} & {\textbf{plant}} & {\textbf{d.table}} & {\textbf{tv}} & {\textbf{All}} \\ \hline
CAM & Image & 68.5 & 49.4 & 22.9 & 16.1 & 54.0 & 37.8 & 24.3 & 51.0 & 31.7 & 47.7 & 40.4 & 39.8 & 49.4 & 45.2 & 40.2 & 50.1 & 22.8 & 22.5 & 39.4 & 33.4 & 34.5 & 39.1 \\
SEAM \cite{wang2020self} & Image & 76.3 & 65.8 & 26.1 & 42.6 & 60.9 & 54.9 & 9.7 & 51.3 & 30.9 & 76.6 & 63.3 & 63.3 & 60.2 & {52.7} & 47.1 & 59.0 & 22.9 & 28.9 & 40.2 & {37.4} & 37.2 & 48.0 \\
SS \cite{araslanov2020single} & Image & 81.8 & 71.2 & 34.8 & 33.7 & {71.3} & {80.7} & 41.7 & {77.5} & 57.2 & 81.1 & 69.2 & {65.6} & 65.0 & 51.3 & {51.4} & 63.7 & 27.6 & 22.8 & {49.5} & 26.4 & 37.8 & 55.3 \\
EPS \cite{lee2021railroad} & Image & 79.9 & 70.2 & 29.0 & {43.1} & 65.3 & 63.2 & {44.3} & 60.7 & 42.4 & 78.6 & {70.3} & 64.6 & 64.4 & 32.2 & 49.4 & {68.1} & 28.2 & {30.0} & 49.4 & 24.9 & 42.6 & 52.4  \\ 
WILSON & Image & {86.6} & {72.9}&	38.1& {46.0}&	67.8&	77.9&	34.4&	55.6&	54.2&	74.2&	74.9&	70.6&	65.2&	66.6&	55.9&	60.1&	29.4&	27.1&	42.4&	21.2&	48.7 & \textbf{55.7}
\end{tabular}
\end{adjustbox}
\caption{Per class results on Pascal VOC for the COCO-to-VOC setting, expressed in mIoU. } \label{tab:coco2voc-voc}
\end{table*}

\begin{table*}[t]

\begin{adjustbox}{width=1.0\textwidth}
\setlength{\tabcolsep}{2pt} 
\begin{tabular}{lcccc|cccccccccccccccc}
\multicolumn{1}{l|}{\textbf{Method}} & \textbf{Old}  & \textbf{New}  & \textbf{All}  & \textbf{bkg} & \textbf{truck}     & \textbf{traffic-light} & \textbf{fire-hydrant} & \textbf{stop-sign} & \textbf{parking-meter} & \textbf{bench}          & \textbf{elephant}   & \textbf{bear}      & \textbf{zebra}         & \textbf{giraffe}    & \textbf{backpack}   & \textbf{umbrella}   & \textbf{handbag} & \textbf{tie}    & \textbf{suitcase} & \textbf{frisbee}     \\ 
\hline
\multicolumn{1}{l|}{CAM}             & 30.7          & 20.3          & 28.1          & 73.8         & 18.3               & 43.7                   & 57.4                  & 87.5               & 35.2                   & 29.3                    & 77.2                & 57.4               & 78.7                   & 66.3                & 10.5                & 35.6                & 2.0              & 3.1             & 47.8              & 0.8                  \\
\multicolumn{1}{l|}{SEAM}            & 31.2          & 28.2          & 30.5          & 81.2         & 15.8               & 40.3                   & 67.5                  & 86.4               & 35.7                   & 30.7                    & 77.3                & 61.6               & 86.8                   & 79.1                & 12.0                & 39.6                & 2.4              & 3.5             & 44.9              & 1.4                  \\
\multicolumn{1}{l|}{SS}              & 35.1          & 36.9          & 35.5          & 81.4         & 13.1               & 47.1                   & 68.9                  & 90.9               & 46.0                   & 28.0                    & 75.4                & 46.1               & 89.3                   & 77.0                & 11.0                & 33.9                & 2.1              & 3.6             & 46.2              & 0.6                  \\
\multicolumn{1}{l|}{EPS}             & 34.9          & \textbf{38.4} & 35.8          & 82.7         & 13.7               & 49.4                   & 67.5                  & 90.9               & 43.6                   & 29.2                    & 77.3                & 49.9               & 87.3                   & 75.9                & 10.2                & 36.3                & 2.1              & 3.8             & 45.7              & 1.1                  \\ 
\multicolumn{1}{l|}{WILSON (Ours)}   & \textbf{36.9} & 37.9          & \textbf{37.2} & 84.9         & 18.4&	58.5&	82.3&	88.8&	67.7&	33.6&	76.5&	54.7&	88.9&	81.1&	13.2&	44.4&	2.1&	4.2&	52.7&	7.1  \\ 
\hline
                                     &               &               &               &              & \textbf{skis}      & \textbf{snowboard}     & \textbf{sports-ball}  & \textbf{kite}      & \textbf{baseball-bat}  & \textbf{baseball-glove} & \textbf{skateboard} & \textbf{surfboard} & \textbf{tennis-racket} & \textbf{wine-glass} & \textbf{cup}        & \textbf{fork}       & \textbf{knife}   & \textbf{spoon}  & \textbf{bowl}     & \textbf{banana}      \\ 
                                     &               &               &               &              & 0.0                & 0.4                    & 5.9                   & 31.9               & 0.0                    & 12.9                    & 1.5                 & 27.0               & 15.8                   & 25.1                & 36.4                & 26.3                & 15.2             & 10.8            & 40.0              & 44.0                 \\
                                     &               &               &               &              & 0.0                & 0.4                    & 5.1                   & 30.8               & 0.0                    & 6.6                     & 0.8                 & 25.7               & 12.2                   & 28.7                & 33.7                & 22.2                & 12.4             & 7.0             & 39.3              & 39.7                 \\
                                     &               &               &               &              & 0.0                & 0.8                    & 1.6                   & 29.2               & 0.0                    & 13.5                    & 0.9                 & 27.0               & 20.2                   & 18.2                & 29.2                & 26.3                & 14.4             & 9.7             & 34.6              & 53.1                 \\
                                     &               &               &               &              & 0.0                & 0.3                    & 5.2                   & 27.6               & 0.0                    & 5.5                     & 1.1                 & 28.2               & 14.5                   & 19.8                & 31.8                & 25.4                & 12.4             & 10.4            & 34.3              & 52.8                 \\ 
                                     &               &               &               &              &	1.8&	0.0&	14.9&	29.3&	0.0&	28.2&	7.7&	28.7&	19.2&	36.1&	37.6&	27.5&	17.3&	16.7&	32.7&	58.1\\ 
\cline{6-21}
                                     &               &               &               &              & \textbf{apple}     & \textbf{sandwich}      & \textbf{orange}       & \textbf{broccoli}  & \textbf{carrot}        & \textbf{hot-dog}        & \textbf{pizza}      & \textbf{donut}     & \textbf{cake}          & \textbf{bed}        & \textbf{toilet}     & \textbf{laptop}     & \textbf{mouse}   & \textbf{remote} & \textbf{keyboard} & \textbf{cell-phone}  \\ 
\cline{6-21}
                                     &               &               &               &              & 33.7               & 30.5                   & 48.7                  & 33.9               & 35.4                   & 39.1                    & 55.7                & 39.0               & 35.1                   & 14.5                & 54.7                & 35.8                & 22.2             & 8.1             & 37.8              & 35.5                 \\
                                     &               &               &               &              & 35.4               & 30.6                   & 50.3                  & 34.9               & 38.4                   & 36.6                    & 54.4                & 37.8               & 38.0                   & 13.9                & 60.8                & 36.2                & 21.3             & 7.0             & 37.4              & 35.2                 \\
                                     &               &               &               &              & 38.1               & 36.7                   & 59.2                  & 47.7               & 49.7                   & 43.6                    & 62.2                & 50.9               & 43.6                   & 20.3                & 69.3                & 41.3                & 34.5             & 28.0            & 45.9              & 35.1                 \\
                                     &               &               &               &              & 39.0               & 38.9                   & 59.2                  & 46.4               & 48.4                   & 44.0                    & 64.3                & 51.6               & 42.2                   & 21.1                & 69.1                & 42.6                & 31.4             & 26.7            & 45.7              & 35.3                 \\ 
                                     &               &               &               &              & 45.7&	40.4&	63.1&	51.7&	48.1&	43.3&	66.6&	55.2&	41.9&	30.8&	72.0&	49.9&	39.9&	34.6&	40.4&	36.7 \\ 
\cline{6-21}
                                     &               &               &               &              & \textbf{microwave} & \textbf{oven}          & \textbf{toaster}      & \textbf{sink}      & \textbf{refrigerator}  & \textbf{book}           & \textbf{clock}      & \textbf{vase}      & \textbf{scissors}      & \textbf{teddy-bear} & \textbf{hair-drier} & \textbf{toothbrush} & \textbf{\color{red}{person}}  & {\color{red}{\textbf{bike}}}   & \textbf{{\color{red}{car}}}      & \textbf{\color{red}{mbike}}       \\ 
\cline{6-21}
                                     &               &               &               &              & 31.9               & 35.6                   & 0.0                   & 28.0               & 42.3                   & 23.2                    & 48.5                & 36.7               & 38.6                   & 55.2                & 0.0                 & 0.0                 & 35.3             & 13.0            & 8.3               & 42.2                 \\
                                     &               &               &               &              & 32.2               & 36.6                   & 0.0                   & 27.6               & 44.2                   & 22.2                    & 51.3                & 37.5               & 44.7                   & 59.5                & 0.0                 & 0.0                 & 59.4             & 17.0            & 10.0              & 46.3                 \\
                                     &               &               &               &              & 34.7               & 50.1                   & 0.0                   & 37.6               & 56.7                   & 24.9                    & 58.3                & 38.1               & 45.0                   & 66.4                & 0.0                 & 29.2                & 67.4             & 43.8            & 17.5              & 57.5                 \\
                                     &               &               &               &              & 33.2               & 50.2                   & 0.0                   & 36.9               & 54.3                   & 24.5                    & 58.7                & 40.0               & 43.7                   & 67.2                & 0.0                 & 27.1                & 70.6             & 40.6            & 9.5               & 61.4                 \\ 
                                     &               &               &               &              & 50.3&	44.7&	3.3&	46.2&	66.4&	31.1&	61.0&	42.8&	46.6&	70.3&	0.0&	33.2&	65.7&	38.4&	25.7&	60.5 \\ 
\cline{6-21}
                                     &               &               &               &              & \textbf{\color{red}{aplane}}    & \textbf{\color{red}{bus}}           & \textbf{\color{red}{train}}        & \textbf{\color{red}{boat}}      & \textbf{\color{red}{bird}}          & \textbf{\color{red}{cat}}            & \textbf{\color{red}{dog}}        & \textbf{\color{red}{horse}}     & \textbf{\color{red}{sheep}}         & \textbf{\color{red}{cow}}        & \textbf{\color{red}{bott}}       & \textbf{\color{red}{chair}}      & \textbf{\color{red}{sofa}}    & \textbf{\color{red}{plant}}  & \textbf{\color{red}{d.table}}  & \textbf{\color{red}{tv}}          \\ 
\cline{6-21}
                                     &               &               &               &              & 12.1               & 15.5                   & 22.9                  & 15.8               & 18.4                   & 37.0                    & 23.0                & 31.9               & 28.6                   & 20.4                & 11.8                & 14.4                & 12.8             & 11.3            & 13.6              & 18.3                 \\
                                     &               &               &               &              & 23.8               & 7.4                    & 19.1                  & 13.1               & 43.9                   & 55.0                    & 41.3                & 49.6               & 39.9                   & 41.2                & 12.4                & 14.9                & 16.8             & 10.2            & 18.2              & 23.5                 \\
                                     &               &               &               &              & 45.7               & 31.9                   & 47.4                  & 27.0               & 41.5                   & 56.0                    & 52.3                & 62.1               & 39.3                   & 48.7                & 20.0                & 13.7                & 17.3             & 12.7            & 11.2              & 24.5                 \\
                                     &               &               &               &              & 52.6               & 27.3                   & 55.7                  & 36.3               & 44.0                   & 57.9                    & 51.4                & 61.3               & 51.1                   & 48.5                & 20.3                & 14.7                & 13.6             & 13.8            & 13.5              & 24.2                 \\ 
                                     &               &               &               &              & 57.8&	26.6&	43.9&	32.9&	51.0&	66.1&	54.9&	64.4&	61.0&	53.5&	25.4&	17.3&	18.9&	14.6&	8.6&	32.5         
\end{tabular}
\end{adjustbox}
\caption{Per class results on COCO for the COCO-to-VOC setting, expressed in mIoU. Best method in bold. VOC classes in red.} 
\label{tab:coco2voc-coco}
\end{table*}
\begin{figure*}[t]
    \centering
    \includegraphics[width=0.95\linewidth]{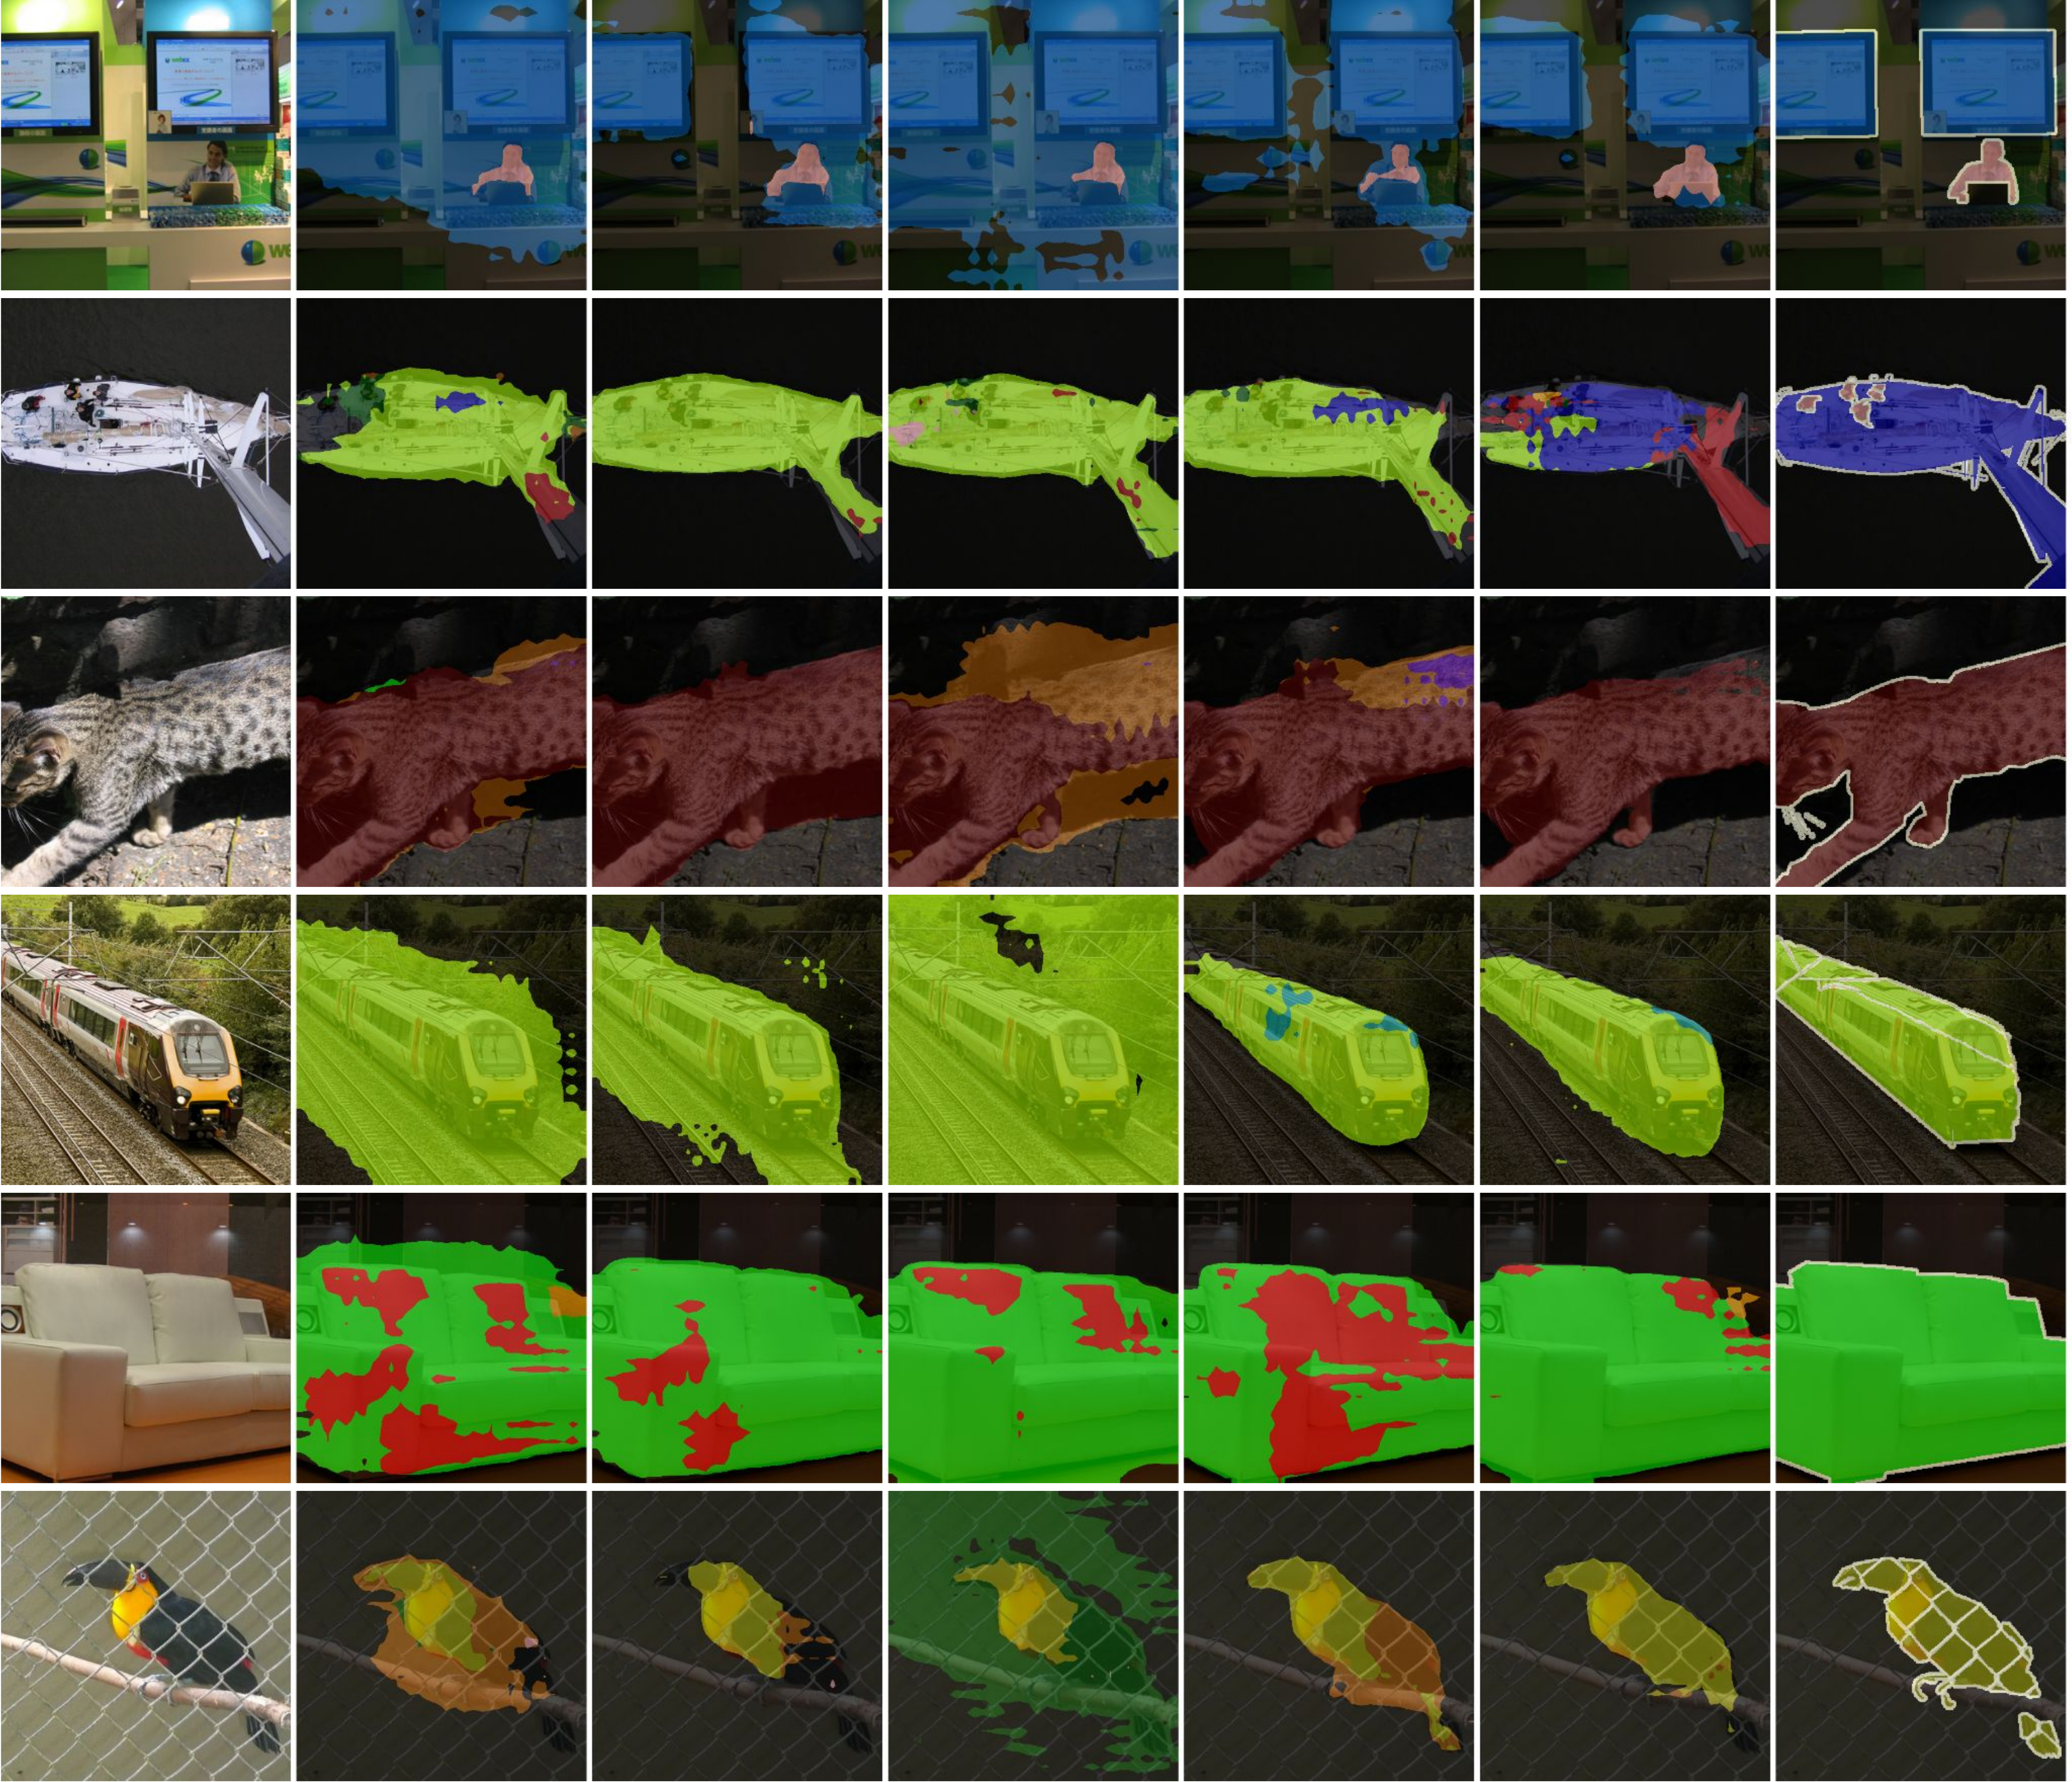}
    \vspace{-5pt}
     \caption{Qualitative results on the 15-5 VOC setting comparing different weakly supervised semantic segmentation methods. From left to right: image, CAM, SEAM \cite{wang2020self}, SS \cite{araslanov2020single}, EPS \cite{lee2021railroad}, \wilson\ and the ground-truth. Best viewed in color.}
    \vspace{-5pt}
    \label{fig:qualitative_15-5}
 \end{figure*}

\begin{figure*}[t]
    \centering
    \includegraphics[width=0.95\linewidth]{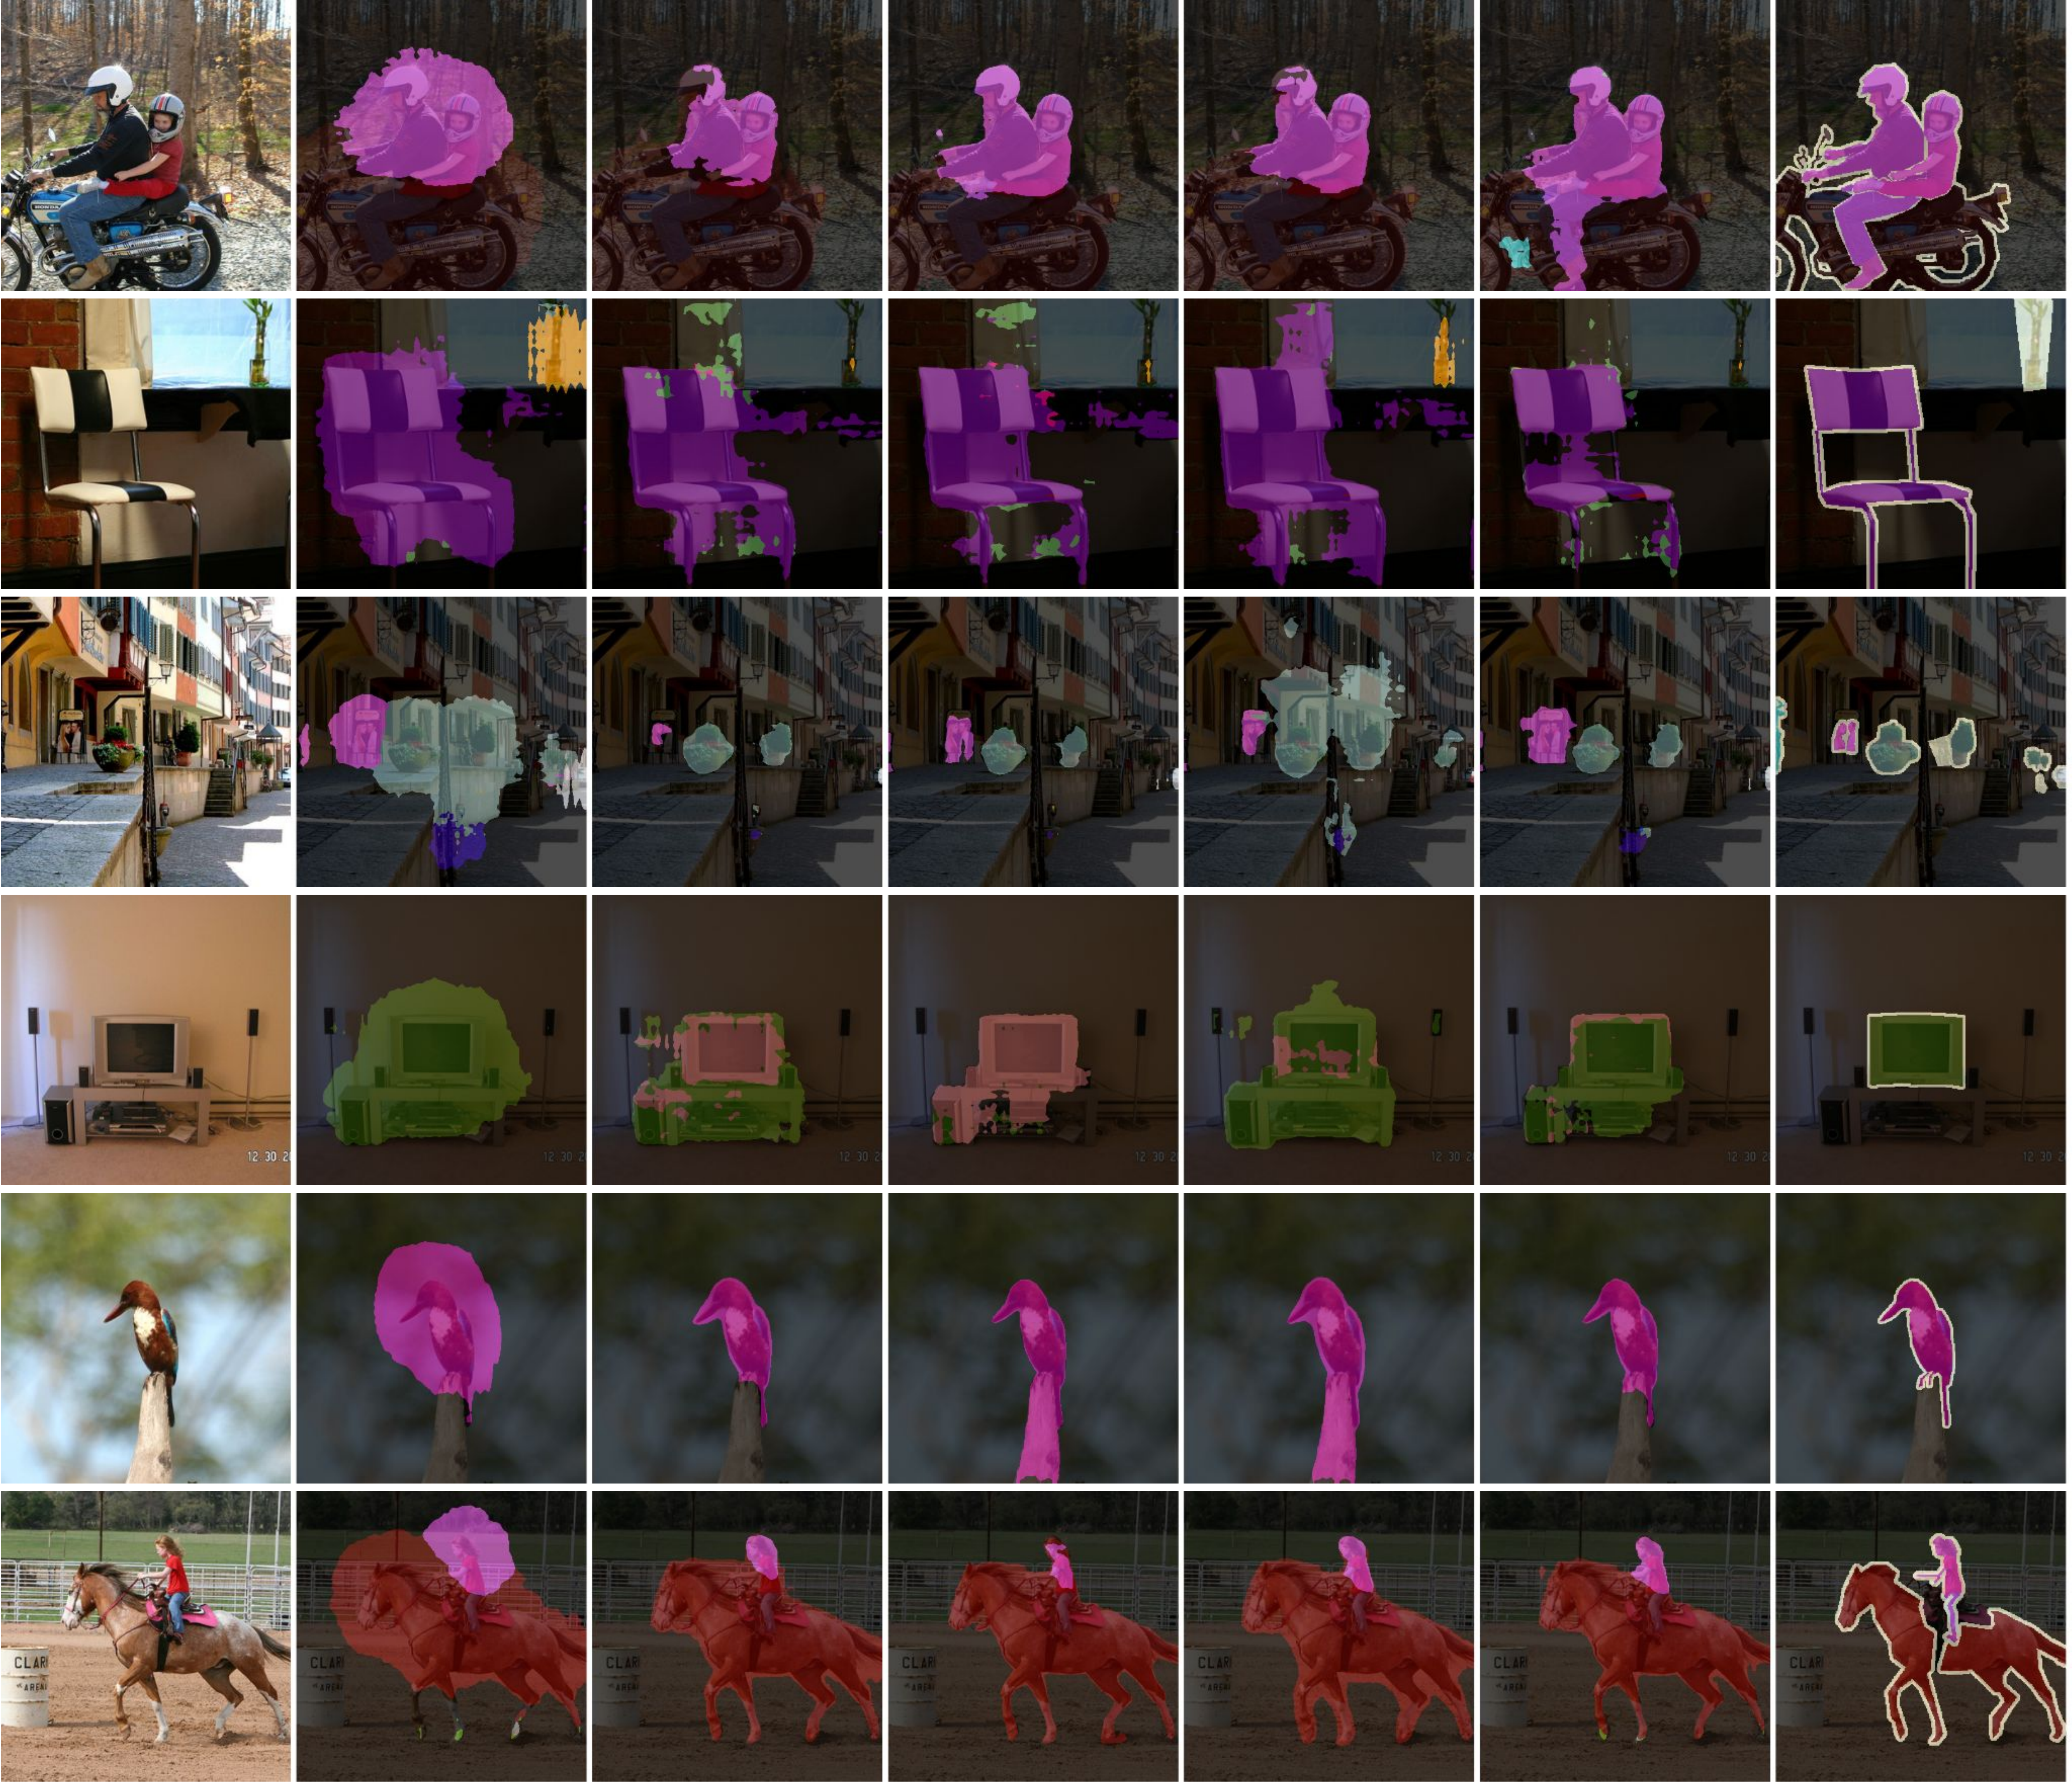}
    \vspace{-5pt}
     \caption{Qualitative results on the COCO-to-VOC setting evaluated on VOC validation set. From left to right: image, CAM, SEAM \cite{wang2020self}, SS \cite{araslanov2020single}, EPS \cite{lee2021railroad}, \wilson\ and the ground-truth. Best viewed in color.}
    \vspace{-5pt}
    \label{fig:qualitative_coco-voc}
 \end{figure*}

\begin{figure*}[t]
    \centering
    \includegraphics[width=0.95\linewidth]{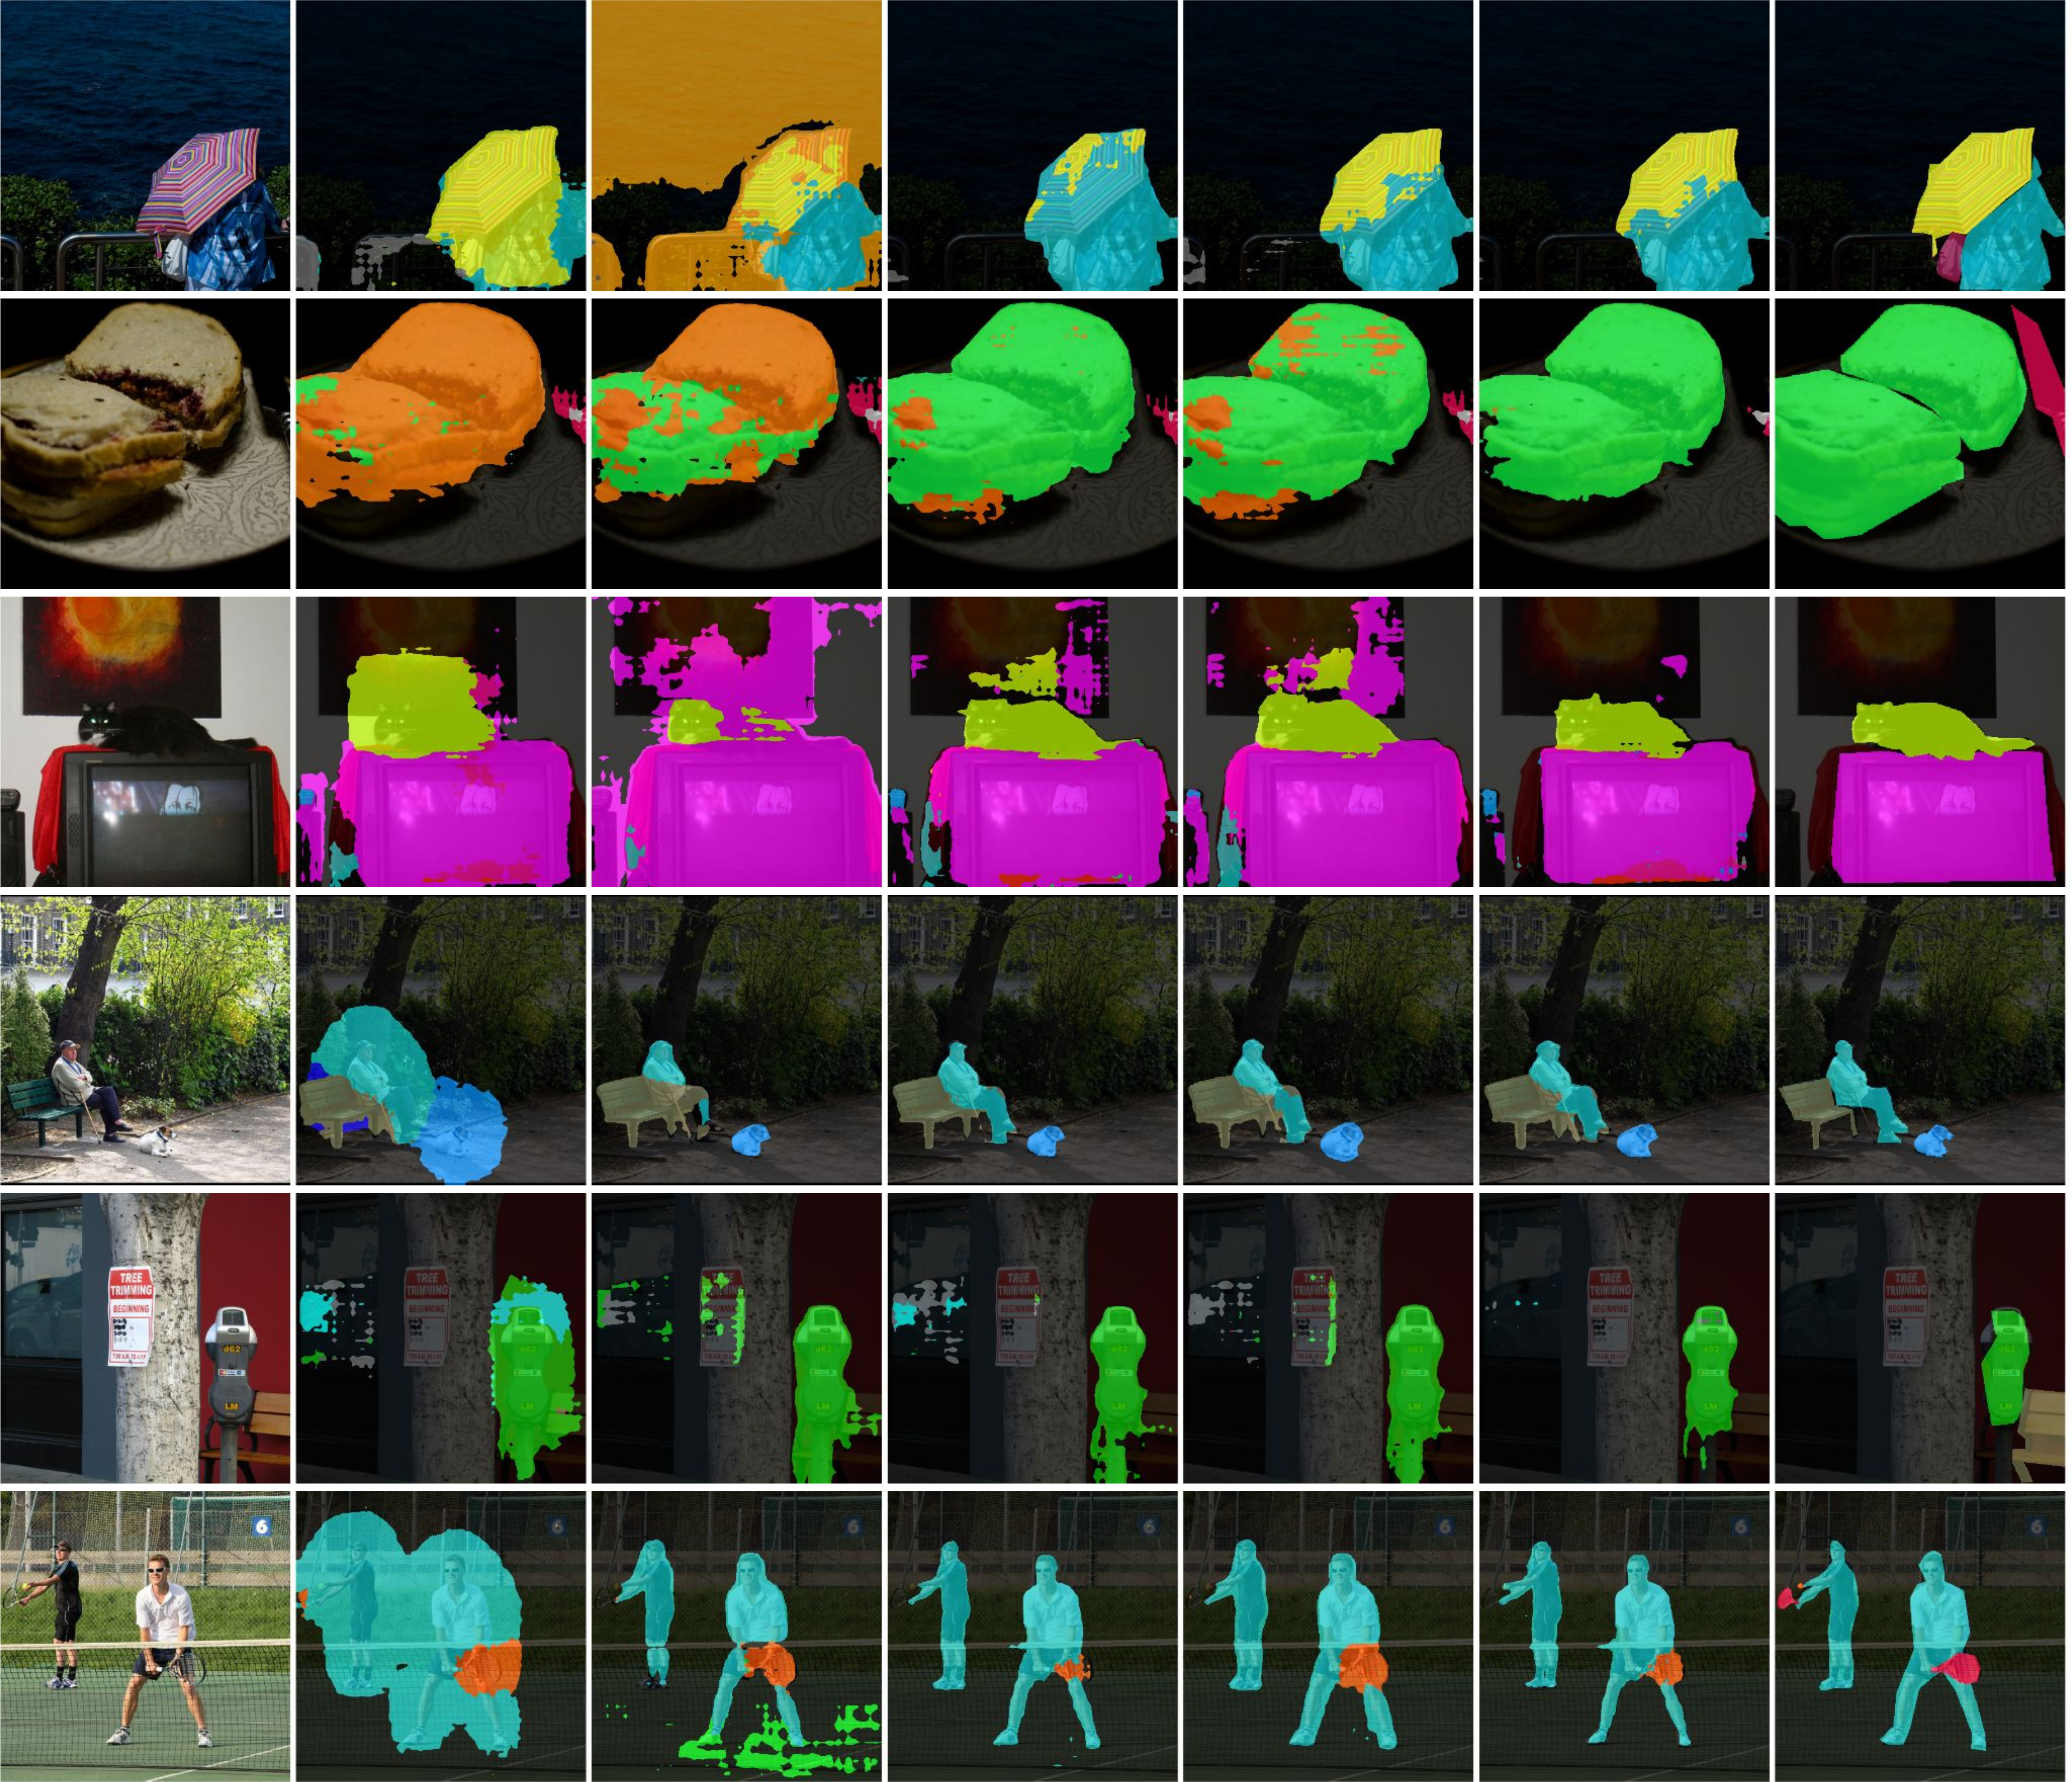}
    \vspace{-5pt}
     \caption{Qualitative results on the COCO-to-VOC setting evaluated on COCO validation set. From left to right: image, CAM, SEAM \cite{wang2020self}, SS \cite{araslanov2020single}, EPS \cite{lee2021railroad}, \wilson\ and the ground-truth. Best viewed in color.}
    \vspace{-5pt}
    \label{fig:qualitative_coco-coco}
 \end{figure*}

\begin{figure*}[t]
    \centering
    \includegraphics[width=0.95\linewidth]{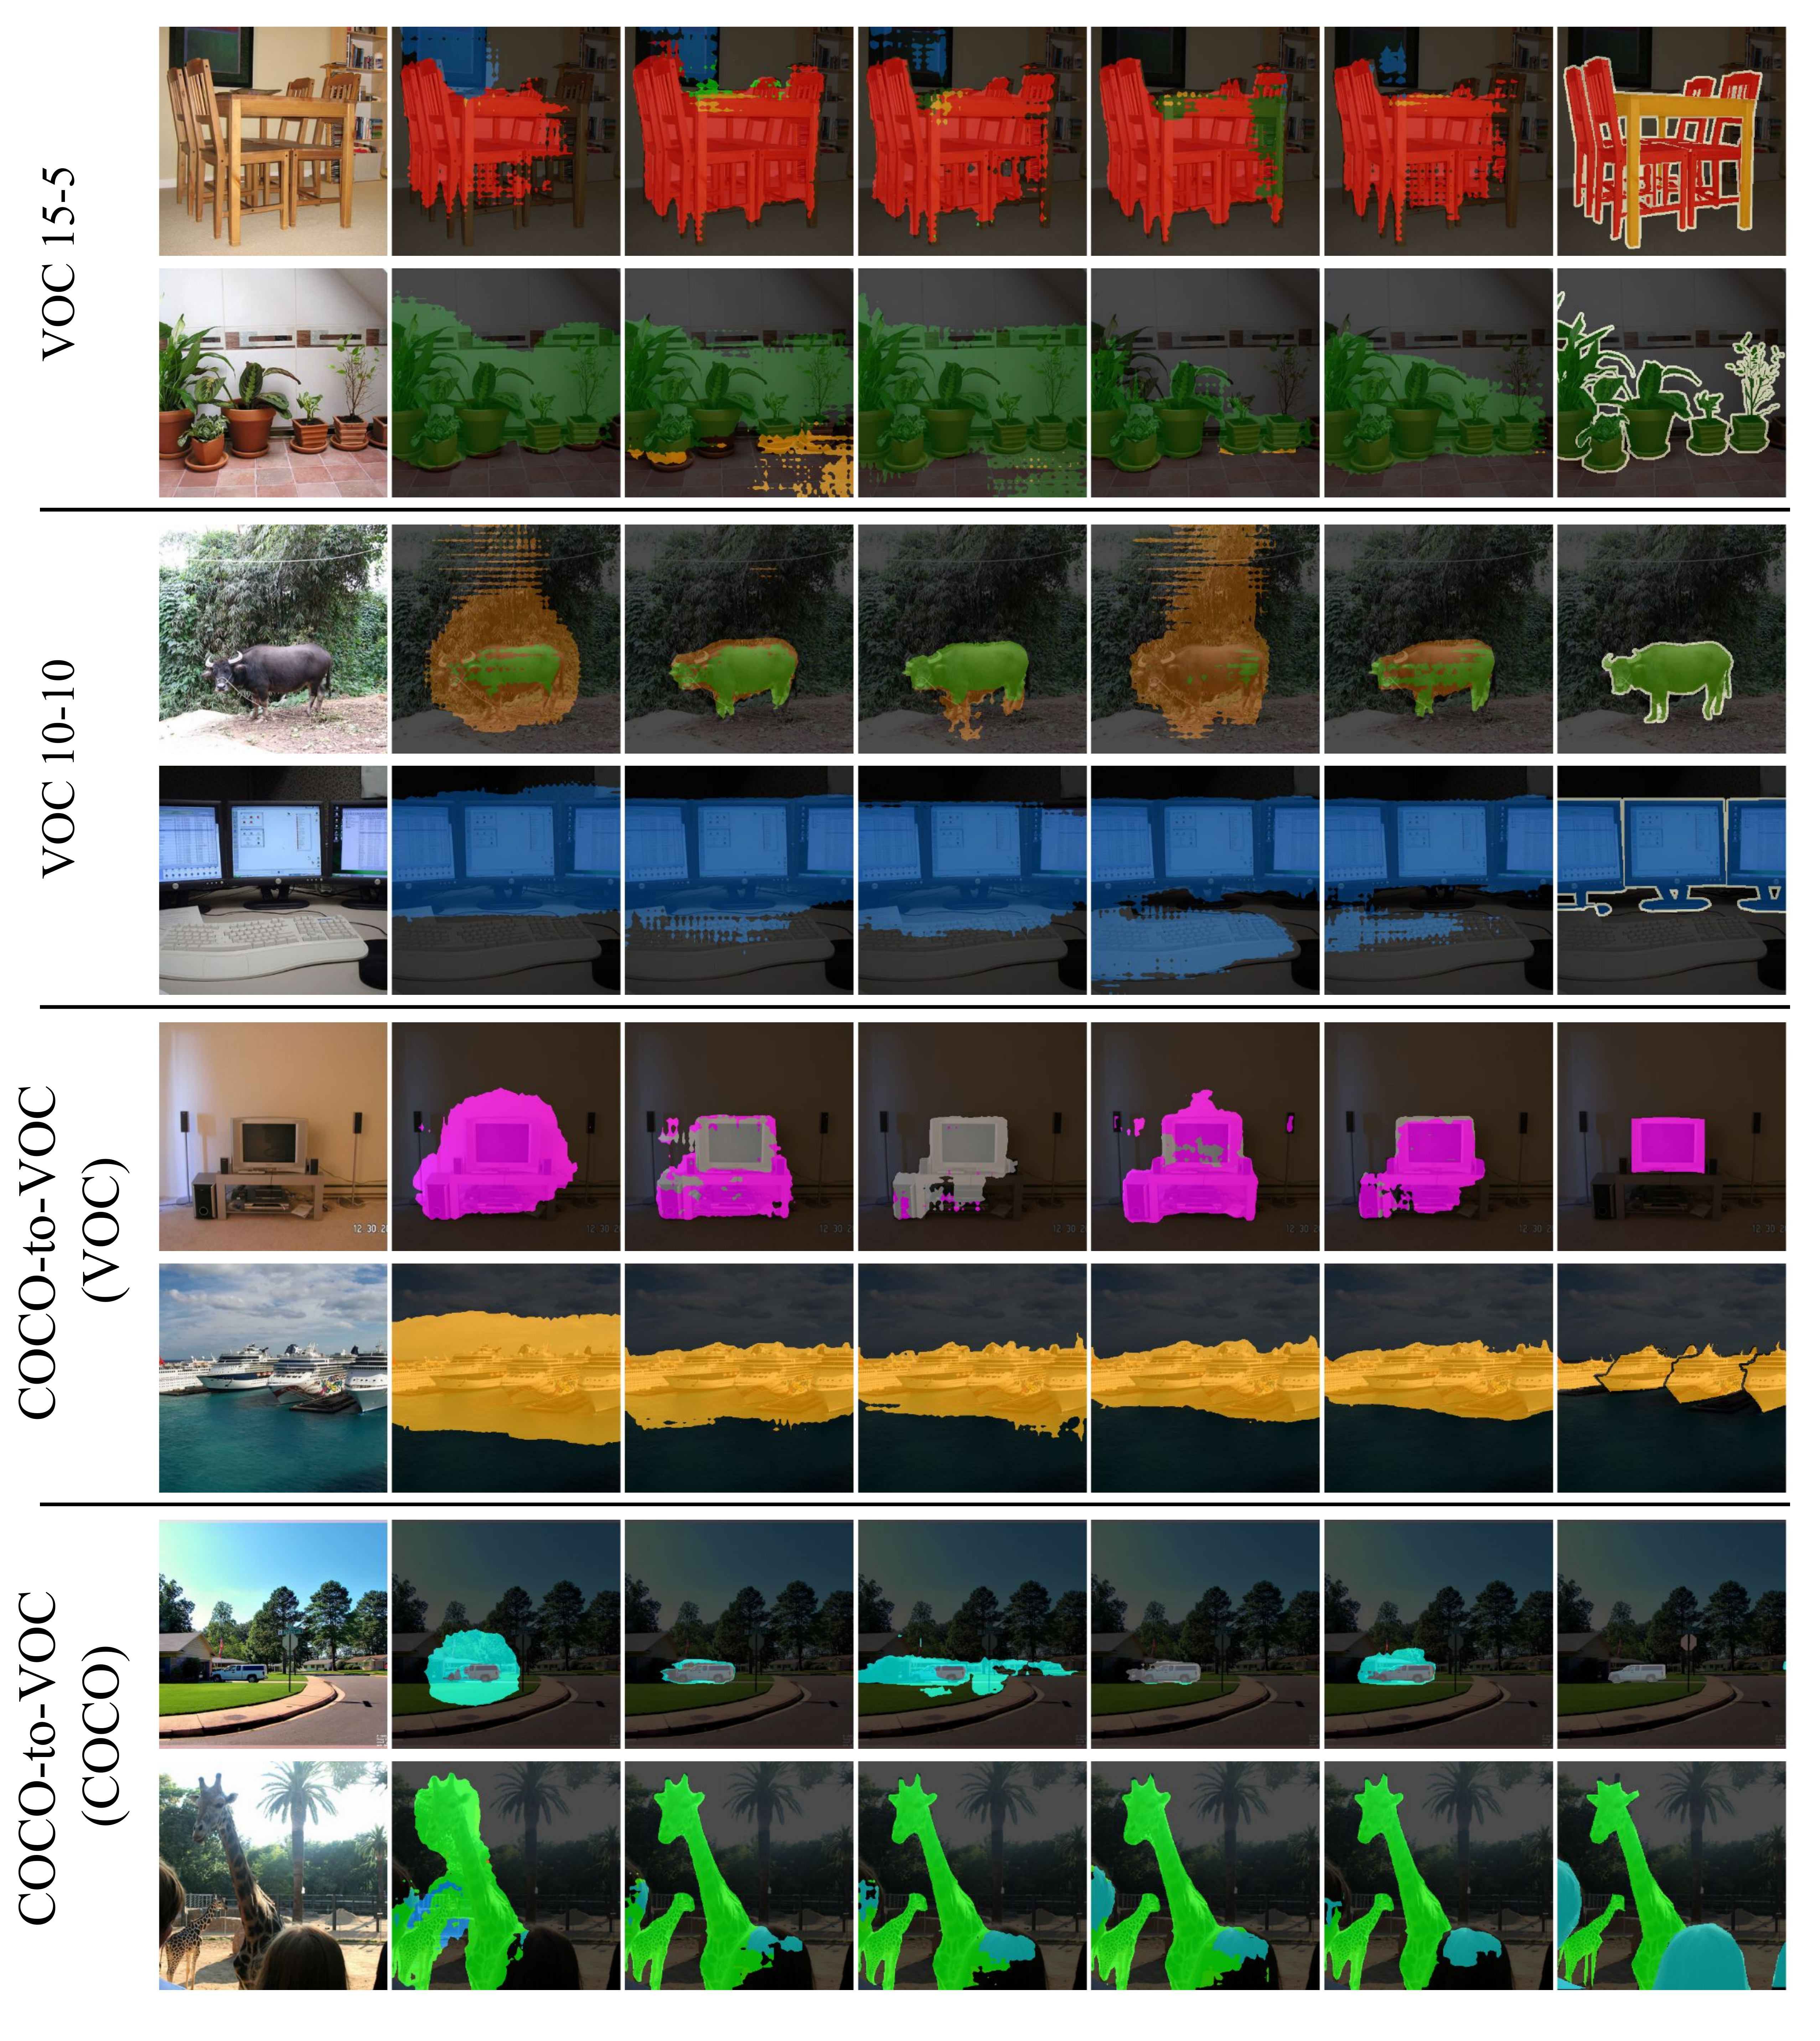}
    \vspace{-5pt}
     \caption{Qualitative results of failure on each setting, in order: VOC 15-5, VOC 10-10, COCO-to-VOC (VOC validation set) and COCO-to-VOC (COCO validation set). From left to right: image, CAM, SEAM \cite{wang2020self}, SS \cite{araslanov2020single}, EPS \cite{lee2021railroad}, \wilson\ and the ground-truth. Best viewed in color.}
    \vspace{-5pt}
    \label{fig:qualitative_failure}
 \end{figure*}

\section{Additional Qualitative Results}
In the main paper, we reported qualitative results for the VOC 10-10 setting. We introduce additional qualitative results here, showing results for each setting (VOC 15-5 and COCO-to-VOC) and some failure cases.

\myparagraph{Single step addition of five classes (15-5).}
\cref{fig:qualitative_15-5} shows evaluations on the Pascal VOC 15-5 setting in which five classes are added in a single step. 
As we can see from the images, \wilson\ predictions on new classes \textit{sofa, train} and \textit{tv-monitor} are much more accurate than those produced by EPS, even if the latter exploits an off-the-shelf saliency detector to better capture object shapes. The performances are even higher than CAM, SEAM, and SS, which tend to extend the new class predictions over the background pixels inaccurately. On old classes, \wilson\ is significantly more resilient to catastrophic forgetting than the other competitors, being able to properly segment both \textit{boat} and \textit{cat} pixels. It is also worth noting that \wilson\ is the only approach capable of accurately classifying the majority of the old class \textit{boat} pixels, avoiding the uncertainty towards the class \textit{train} that the other competitors manifest.

\myparagraph{COCO-to-VOC.}
\cref{fig:qualitative_coco-voc} and \cref{fig:qualitative_coco-coco} provide the results on COCO-to-VOC setting in which additional 20 VOC classes are added in a second step, respectively evaluating each method on VOC and COCO validation sets.
\cref{fig:qualitative_coco-voc} confirms the strong performances on newer classes observed in the VOC 15-5 and 10-10 settings, demonstrating how only \wilson\ is able to segment the leg of the motorcyclist and the background of the \textit{chair} with significantly fewer inaccuracies than the others competitors. The results achieved on \textit{plant} category show the ability of \wilson\ in successfully segmenting small objects as well, compared to EPS which entirely fails in accurately predicting small object boundaries.
Even on the COCO validation dataset, \wilson\ outperforms the other state-of-the-art weakly-supervised semantic segmentation methods, as shown in \cref{fig:qualitative_coco-coco}. Indeed, it is able to segment the old classes \textit{umbrella, sandwich, parking meter} and the new ones \textit{person, dog, cat, tv-monitor} with much less uncertainty. Both CAM and SS perform poorly in this scenario, while SEAM and EPS still show some misclassified pixels. We also note that none of the provided approaches can classify the \textit{tennis racket} correctly. We attribute this behavior to a context bias, as many training images involve a person holding a skateboard, and the models have learned to associate a person holding \textit{something} to a \textit{skateboard}.

\myparagraph{Failure Modes.}
Finally, \cref{fig:qualitative_failure} reports some failure cases and inaccurate predictions of each method. 
{The first situation in which \wilson\ exhibits difficulties is in separating the object from its context}. Indeed, like with the \textit{table-chair} pair in VOC 15-5, \textit{monitor-keyboard} in VOC 10-10, and \textit{tv-monitor-furniture} in COCO-to-VOC (VOC), {it includes in the prediction of the main class also objects that are commonly observed together.} The second flaw regards object boundaries. \wilson\, as shown in VOC 15-5, is unable to appropriately segment each boundary of the new class \textit{plant}, whereas EPS is able to do so. The same trend may be seen in COCO-to-VOC (VOC) \textit{boat}. Finally, \wilson\ demonstrates the final failure in terms of misclassified predictions between old and new classes. It mixes the old class \textit{sheep} with the new class \textit{cow}, as illustrated in VOC 10-10. Furthermore, it confuses \textit{truck} and \textit{car} in COCO-to-VOC (COCO).
