# Supplementary material for: Incremental Learning in Semantic Segmentation from Image Labels
Source: arXiv:2112.01882 source file (2022-03-31)
Supplement: Supplementary file 2 [file supp.tex]

\begin{table*}[t]

\begin{adjustbox}{width=1.0\textwidth}
\setlength{\tabcolsep}{3pt} 
\begin{tabular}{lc|cccccccccccccccc|ccccc|ccc}
\textbf{Method} & \textbf{Sup} & \textbf{bkg} & \textbf{aplane} & \textbf{bike} & \textbf{bird} & \textbf{boat} & \textbf{bott} & \textbf{bus} & \textbf{car} & \textbf{cat} & \textbf{chair} & \textbf{cow} & \textbf{d.table} & \textbf{dog} & \textbf{horse} & \textbf{mbike} & \textbf{person} & \textbf{plant} & \textbf{sheep} & \textbf{sofa} & \textbf{train} & \textbf{tv} & \textbf{Old} & \textbf{New} & \textbf{All} \\ \hline
Joint & Pixel & 92.5 & 89.9 & 39.2 & 87.6 & 65.2 & 77.3 & 91.1 & 88.5 & 92.9 & 34.8 & 84.0 & 53.7 & 88.9 & 85.0 & 85.1 & 84.9 & 60.0 & 79.7 & 47.0 & 82.2 & 73.5 & 76.5 & 68.5 & 75.4 \\ \hline
CAM                           & Image & 77.6&	74.9&	38.5&	73.5&	60.0&	72.4&	81.6&	86.7&	89.7&	32.4&	42.0&	56.0&	85.5&	77.8&	84.3&	84.6&	20.7&	15.9&	27.9&	32.7&	33.2&		69.3&	26.1&	59.4 \\
SEAM \cite{wang2020self}      & Image & 86.3&	79.6&	39.5&	81.3&	54.0&	66.0&	81.3&	85.2&	88.8&	34.2&	64.8&	56.2&	87.6&	80.2&	82.5&	84.5&	17.7&	36.6&	29.9&	45.2&	35.9&		71.0&	33.1&	62.7 \\
SS \cite{araslanov2020single} & Image & 86.4&	77.2&	38.7&	83.2&	62.0&	75.9&	76.5&	88.3&	89.1&	33.3&	63.1&	57.9&	84.0&	80.9&	79.9&	84.2&	18.6&	22.4&	20.3&	26.8&	41.9&		71.6&	26.0&	61.5 \\
EPS \cite{lee2021railroad}    & Image & 90.2&	83.9&	40.8&	84.9&	63.9&	75.7&	83.6&	86.9&	89.8&	34.0&	52.3&	56.4&	87.6&	82.6&	80.1&	83.9&	20.1&	43.9&	23.8&	64.8&	39.8&		72.4&	38.5&	65.2 \\
WILSON (Ours)                 & Image & 90.5&	88.8&	40.9&	86.4&	69.4&	77.9&	82.9&	88.0&	92.3&	35.4&	51.3&	56.2&	88.3&	83.9&	77.2&	85.1&	30.3&	47.5&	39.2&	54.6&	47.5&		\textbf{73.6}&	\textbf{43.8}&	\textbf{67.3} \\
\end{tabular}
\end{adjustbox}
\caption{Per class results on the Pascal VOC 15-5 Disjoint setting, expressed in mIoU. Best Image-supervised method in bold.} \label{tab:voc-15-5-d}
\end{table*}

\begin{table*}[t]

\begin{adjustbox}{width=1.0\textwidth}
\setlength{\tabcolsep}{3pt} 
\begin{tabular}{lc|cccccccccccccccc|ccccc|ccc}
\textbf{Method} & \textbf{Sup} & \textbf{bkg} & \textbf{plane} & \textbf{bike} & \textbf{bird} & \textbf{boat} & \textbf{bottle} & \textbf{bus} & \textbf{car} & \textbf{cat} & \textbf{chair} & \textbf{cow} & \textbf{d.table} & \textbf{dog} & \textbf{horse} & \textbf{m.bike} & \textbf{person} & \textbf{plant} & \textbf{sheep} & \textbf{sofa} & \textbf{train} & \textbf{tv} & \textbf{Old} & \textbf{New} & \textbf{All} \\ \hline
Joint & Pixel & 92.5 & 89.9 & 39.2 & 87.6 & 65.2 & 77.3 & 91.1 & 88.5 & 92.9 & 34.8 & 84.0 & 53.7 & 88.9 & 85.0 & 85.1 & 84.9 & 60.0 & 79.7 & 47.0 & 82.2 & 73.5 & 76.5 & 68.5 & 75.4 \\ \hline
CAM                           & Image & 77.0&	75.2&	38.3&	77.3&	60.5&	74.9&	71.3&	85.3&	88.4&	35.4&	54.8&	53.9&	86.5&	80.7&	81.2&	84.3&	16.6&	15.1&	28.3&	35.2&	33.0&		69.9&	25.6&	59.7 \\
SEAM \cite{wang2020self}      & Image & 85.3&	77.5&	39.6&	78.9&	53.9&	61.2&	58.7&	83.4&	87.8&	36.3&	69.6&	49.7&	86.3&	81.0&	76.9&	84.1&	13.0&	38.1&	29.8&	41.6&	36.2&		68.3&	31.8&	60.4 \\
SS \cite{araslanov2020single} & Image & 84.9&	78.7&	38.0&	82.2&	61.7&	74.9&	79.3&	85.4&	88.0&	40.1&	70.4&	56.9&	82.4&	81.7&	78.5&	84.3&	13.4&	27.4&	26.0&	32.7&	38.0&		72.2&	27.5&	62.1 \\
EPS \cite{lee2021railroad}    & Image & 89.6&	81.7&	39.4&	81.8&	63.6&	73.9&	53.2&	84.6&	88.1&	38.9&	53.1&	57.1&	86.8&	80.9&	74.0&	83.7&	16.4&	39.9&	27.8&	51.9&	36.7&		69.4&	34.5&	62.1 \\
WILSON (Ours)                 & Image & 89.5&	88.6&	41.2&	84.9&	68.7&	79.0&	83.9&	88.5&	91.7&	39.3&	55.7&	58.3&	89.0&	85.7&	73.3&	85.8&	26.5&	48.6&	36.6&	55.7&	40.9&		\textbf{74.2}&	\textbf{41.7}&	\textbf{67.2} \\
\end{tabular}
\end{adjustbox}
\caption{Per class results on the Pascal VOC 15-5 Overlapped setting, expressed in mIoU. Best Image-supervised method in bold.} \label{tab:voc-15-5-o}
\end{table*}

\begin{table*}[t]

\begin{adjustbox}{width=1.0\textwidth}
\setlength{\tabcolsep}{3pt} 
\begin{tabular}{lc|ccccccccccc|cccccccccc|ccc}
\textbf{Method} & \textbf{Sup} & \textbf{bkg} & \textbf{aplane} & \textbf{bike} & \textbf{bird} & \textbf{boat} & \textbf{bott} & \textbf{bus} & \textbf{car} & \textbf{cat} & \textbf{chair} & \textbf{cow} & \textbf{d.table} & \textbf{dog} & \textbf{horse} & \textbf{mbike} & \textbf{person} & \textbf{plant} & \textbf{sheep} & \textbf{sofa} & \textbf{train} & \textbf{tv} & \textbf{Old} & \textbf{New} & \textbf{All} \\
\hline 
Joint & Pixel & 92.5 & 89.9 & 39.2 & 87.6 & 65.2 & 77.3 & 91.1 & 88.5 & 92.9 & 34.8 & 84.0 & 53.7 & 88.9 & 85.0 & 85.1 & 84.9 & 60.0 & 79.7 & 47.0 & 82.2 & 73.5 & 75.1 & 74.0 & 75.4 \\
\hline 
CAM                           & Image & 78.5&	87.9&	35.6&	81.6&	62.3&	77.9&	76.6&	78.1&	73.1&	24.5&	56.1&	38.1&	41.9&	28.9&	50.2&	47.5&	37.6&	40.0&	34.1&	49.0&	45.2&		\textbf{65.4}&	41.3&	54.5\\
SEAM \cite{wang2020self}      & Image & 87.4&	88.8&	35.7&	84.4&	63.5&	77.2&	71.4&	66.6&	76.4&	27.6&	59.3&	42.1&	65.2&	45.6&	64.3&	59.3&	37.9&	67.9&	44.5&	56.1&	52.5&		65.1&	53.5&	60.7 \\
SS \cite{araslanov2020single} & Image & 81.2&	81.5&	25.3&	85.4&	64.5&	80.5&	78.0&	68.4&	60.1&	25.4&	38.4&	14.8&	17.2&	6.4&	26.1&	24.4&	29.7&	33.8&	21.1&	38.5&	45.5&		60.8&	25.7&	45.1 \\
EPS \cite{lee2021railroad}    & Image & 89.1&	79.2&	35.3&	85.2&	66.8&	80.2&	61.1&	70.6&	77.4&	26.0&	60.3&	38.1&	64.8&	51.1&	68.7&	66.8&	43.4&	50.8&	39.4&	73.8&	44.5&		64.2&	54.1&	60.6\\  
WILSON (Ours)                 & Image & 89.7&	78.8&	33.1&	87.7&	57.8&	80.9&	75.5&	71.3&	75.7&	28.7&	55.0&	27.7&	66.8&	43.3&	64.3&	59.5&	45.9&	63.2&	37.6&	74.3&	60.4&		64.5&	\textbf{54.3}&	\textbf{60.8}    
\end{tabular}
\end{adjustbox}
\caption{Per class results on the Pascal VOC 10-10 Disjoint setting, expressed in mIoU. Best Image-supervised method in bold.} \label{tab:voc-10-10-d}
\end{table*}

\begin{table*}[t]

\begin{adjustbox}{width=1.0\textwidth}
\setlength{\tabcolsep}{3pt} 
\begin{tabular}{lc|ccccccccccc|cccccccccc|ccc}
\textbf{Method} & \textbf{Sup} & \textbf{bkg} & \textbf{aplane} & \textbf{bike} & \textbf{bird} & \textbf{boat} & \textbf{bott} & \textbf{bus} & \textbf{car} & \textbf{cat} & \textbf{chair} & \textbf{cow} & \textbf{d.table} & \textbf{dog} & \textbf{horse} & \textbf{mbike} & \textbf{person} & \textbf{plant} & \textbf{sheep} & \textbf{sofa} & \textbf{train} & \textbf{tv} & \textbf{Old} & \textbf{New} & \textbf{All} \\
\hline 
Joint & Pixel & 92.5 & 89.9 & 39.2 & 87.6 & 65.2 & 77.3 & 91.1 & 88.5 & 92.9 & 34.8 & 84.0 & 53.7 & 88.9 & 85.0 & 85.1 & 84.9 & 60.0 & 79.7 & 47.0 & 82.2 & 73.5 & 75.1 & 74.0 & 75.4 \\
\hline
CAM                           & Image &78.4&	85.9&	38.7&	82.9&	68.4&	78.9&	82.7&	85.6&	83.0&	34.2&	67.5&	39.0&	51.1&	40.5&	53.7&	48.0&	39.1&	39.0&	37.1&	50.1&	44.5&		\textbf{70.8}&	44.2&	58.5 \\
SEAM \cite{wang2020self}      & Image &87.1&	84.2&	38.5&	84.4&	63.3&	77.2&	71.7&	69.6&	83.1&	33.7&	69.8&	44.5&	73.8&	60.5&	67.3&	59.2&	38.0&	65.1&	41.3&	54.9&	49.3&		67.5&	55.4&	62.7 \\
SS \cite{araslanov2020single} & Image &79.1&	85.8&	38.3&	84.1&	67.1&	79.4&	84.5&	84.8&	78.8&	34.0&	59.1&	17.4&	40.6&	31.9&	40.5&	23.6&	29.9&	37.9&	24.0&	38.4&	44.1&		69.6&	32.8&	52.5 \\
EPS \cite{lee2021railroad}    & Image &88.9&	87.3&	37.7&	84.4&	68.7&	77.6&	66.0&	75.5&	84.8&	35.8&	72.8&	38.9&	76.2&	65.5&	73.7&	66.7&	42.4&	50.8&	38.9&	76.0&	41.9&		69.0&	{57.0}&	64.3 \\
WILSON (Ours)                 & Image &89.1&	83.6&	38.1&	86.5&	62.8&	79.6&	79.3&	83.7&	85.4&	33.0&	72.3&	29.0&	77.8&	64.5&	73.9&	59.8&	40.9&	67.9&	37.5&	57.0&	62.3&		70.4&	\textbf{57.1}&	\textbf{65.0} \\

\end{tabular}
\end{adjustbox}
\caption{Per class results on the Pascal VOC 10-10 Overlapped setting, expressed in mIoU. Best Image-supervised method in bold.} \label{tab:voc-10-10-o}
\end{table*}

\begin{table*}[t]

\begin{adjustbox}{width=1.0\textwidth}
\setlength{\tabcolsep}{3pt} 
\begin{tabular}{lc|ccccccccccccccccccccc|c}
{\textbf{Method}} & \textbf{Sup} & {\textbf{bkg}} & {\textbf{person}} & {\textbf{bike}} & {\textbf{car}} & {\textbf{mbike}} & {\textbf{aplane}} & {\textbf{bus}} & {\textbf{train}} & {\textbf{boat}} & {\textbf{bird}} & {\textbf{cat}} & {\textbf{dog}} & {\textbf{horse}} & {\textbf{sheep}} & {\textbf{cow}} & {\textbf{bott}} & {\textbf{chair}} & {\textbf{sofa}} & {\textbf{plant}} & {\textbf{d.table}} & {\textbf{tv}} & {\textbf{All}} \\ \hline
CAM & Image & 68.5 & 49.4 & 22.9 & 16.1 & 54.0 & 37.8 & 24.3 & 51.0 & 31.7 & 47.7 & 40.4 & 39.8 & 49.4 & 45.2 & 40.2 & 50.1 & 22.8 & 22.5 & 39.4 & 33.4 & 34.5 & 39.1 \\
SEAM \cite{wang2020self} & Image & 76.3 & 65.8 & 26.1 & 42.6 & 60.9 & 54.9 & 9.7 & 51.3 & 30.9 & 76.6 & 63.3 & 63.3 & 60.2 & {52.7} & 47.1 & 59.0 & 22.9 & 28.9 & 40.2 & {37.4} & 37.2 & 48.0 \\
SS \cite{araslanov2020single} & Image & 81.8 & 71.2 & 34.8 & 33.7 & {71.3} & {80.7} & 41.7 & {77.5} & 57.2 & 81.1 & 69.2 & {65.6} & 65.0 & 51.3 & {51.4} & 63.7 & 27.6 & 22.8 & {49.5} & 26.4 & 37.8 & 55.3 \\
EPS \cite{lee2021railroad} & Image & 79.9 & 70.2 & 29.0 & {43.1} & 65.3 & 63.2 & {44.3} & 60.7 & 42.4 & 78.6 & {70.3} & 64.6 & 64.4 & 32.2 & 49.4 & {68.1} & 28.2 & {30.0} & 49.4 & 24.9 & 42.6 & 52.4  \\ 
WILSON & Image & {86.6} & {72.9}&	38.1& {46.0}&	67.8&	77.9&	34.4&	55.6&	54.2&	74.2&	74.9&	70.6&	65.2&	66.6&	55.9&	60.1&	29.4&	27.1&	42.4&	21.2&	48.7 & \textbf{55.7}
\end{tabular}
\end{adjustbox}
\caption{Per class results on Pascal VOC for the COCO-to-VOC setting, expressed in mIoU. } \label{tab:coco2voc-voc}
\end{table*}

\begin{table*}[t]

\begin{adjustbox}{width=1.0\textwidth}
\setlength{\tabcolsep}{2pt} 
\begin{tabular}{lcccc|cccccccccccccccc}
\multicolumn{1}{l|}{\textbf{Method}} & \textbf{Old}  & \textbf{New}  & \textbf{All}  & \textbf{bkg} & \textbf{truck}     & \textbf{traffic-light} & \textbf{fire-hydrant} & \textbf{stop-sign} & \textbf{parking-meter} & \textbf{bench}          & \textbf{elephant}   & \textbf{bear}      & \textbf{zebra}         & \textbf{giraffe}    & \textbf{backpack}   & \textbf{umbrella}   & \textbf{handbag} & \textbf{tie}    & \textbf{suitcase} & \textbf{frisbee}     \\ 
\hline
\multicolumn{1}{l|}{CAM}             & 30.7          & 20.3          & 28.1          & 73.8         & 18.3               & 43.7                   & 57.4                  & 87.5               & 35.2                   & 29.3                    & 77.2                & 57.4               & 78.7                   & 66.3                & 10.5                & 35.6                & 2.0              & 3.1             & 47.8              & 0.8                  \\
\multicolumn{1}{l|}{SEAM}            & 31.2          & 28.2          & 30.5          & 81.2         & 15.8               & 40.3                   & 67.5                  & 86.4               & 35.7                   & 30.7                    & 77.3                & 61.6               & 86.8                   & 79.1                & 12.0                & 39.6                & 2.4              & 3.5             & 44.9              & 1.4                  \\
\multicolumn{1}{l|}{SS}              & 35.1          & 36.9          & 35.5          & 81.4         & 13.1               & 47.1                   & 68.9                  & 90.9               & 46.0                   & 28.0                    & 75.4                & 46.1               & 89.3                   & 77.0                & 11.0                & 33.9                & 2.1              & 3.6             & 46.2              & 0.6                  \\
\multicolumn{1}{l|}{EPS}             & 34.9          & \textbf{38.4} & 35.8          & 82.7         & 13.7               & 49.4                   & 67.5                  & 90.9               & 43.6                   & 29.2                    & 77.3                & 49.9               & 87.3                   & 75.9                & 10.2                & 36.3                & 2.1              & 3.8             & 45.7              & 1.1                  \\ 
\multicolumn{1}{l|}{WILSON (Ours)}   & \textbf{36.9} & 37.9          & \textbf{37.2} & 84.9         & 18.4&	58.5&	82.3&	88.8&	67.7&	33.6&	76.5&	54.7&	88.9&	81.1&	13.2&	44.4&	2.1&	4.2&	52.7&	7.1  \\ 
\hline
                                     &               &               &               &              & \textbf{skis}      & \textbf{snowboard}     & \textbf{sports-ball}  & \textbf{kite}      & \textbf{baseball-bat}  & \textbf{baseball-glove} & \textbf{skateboard} & \textbf{surfboard} & \textbf{tennis-racket} & \textbf{wine-glass} & \textbf{cup}        & \textbf{fork}       & \textbf{knife}   & \textbf{spoon}  & \textbf{bowl}     & \textbf{banana}      \\ 
                                     &               &               &               &              & 0.0                & 0.4                    & 5.9                   & 31.9               & 0.0                    & 12.9                    & 1.5                 & 27.0               & 15.8                   & 25.1                & 36.4                & 26.3                & 15.2             & 10.8            & 40.0              & 44.0                 \\
                                     &               &               &               &              & 0.0                & 0.4                    & 5.1                   & 30.8               & 0.0                    & 6.6                     & 0.8                 & 25.7               & 12.2                   & 28.7                & 33.7                & 22.2                & 12.4             & 7.0             & 39.3              & 39.7                 \\
                                     &               &               &               &              & 0.0                & 0.8                    & 1.6                   & 29.2               & 0.0                    & 13.5                    & 0.9                 & 27.0               & 20.2                   & 18.2                & 29.2                & 26.3                & 14.4             & 9.7             & 34.6              & 53.1                 \\
                                     &               &               &               &              & 0.0                & 0.3                    & 5.2                   & 27.6               & 0.0                    & 5.5                     & 1.1                 & 28.2               & 14.5                   & 19.8                & 31.8                & 25.4                & 12.4             & 10.4            & 34.3              & 52.8                 \\ 
                                     &               &               &               &              &	1.8&	0.0&	14.9&	29.3&	0.0&	28.2&	7.7&	28.7&	19.2&	36.1&	37.6&	27.5&	17.3&	16.7&	32.7&	58.1\\ 
\cline{6-21}
                                     &               &               &               &              & \textbf{apple}     & \textbf{sandwich}      & \textbf{orange}       & \textbf{broccoli}  & \textbf{carrot}        & \textbf{hot-dog}        & \textbf{pizza}      & \textbf{donut}     & \textbf{cake}          & \textbf{bed}        & \textbf{toilet}     & \textbf{laptop}     & \textbf{mouse}   & \textbf{remote} & \textbf{keyboard} & \textbf{cell-phone}  \\ 
\cline{6-21}
                                     &               &               &               &              & 33.7               & 30.5                   & 48.7                  & 33.9               & 35.4                   & 39.1                    & 55.7                & 39.0               & 35.1                   & 14.5                & 54.7                & 35.8                & 22.2             & 8.1             & 37.8              & 35.5                 \\
                                     &               &               &               &              & 35.4               & 30.6                   & 50.3                  & 34.9               & 38.4                   & 36.6                    & 54.4                & 37.8               & 38.0                   & 13.9                & 60.8                & 36.2                & 21.3             & 7.0             & 37.4              & 35.2                 \\
                                     &               &               &               &              & 38.1               & 36.7                   & 59.2                  & 47.7               & 49.7                   & 43.6                    & 62.2                & 50.9               & 43.6                   & 20.3                & 69.3                & 41.3                & 34.5             & 28.0            & 45.9              & 35.1                 \\
                                     &               &               &               &              & 39.0               & 38.9                   & 59.2                  & 46.4               & 48.4                   & 44.0                    & 64.3                & 51.6               & 42.2                   & 21.1                & 69.1                & 42.6                & 31.4             & 26.7            & 45.7              & 35.3                 \\ 
                                     &               &               &               &              & 45.7&	40.4&	63.1&	51.7&	48.1&	43.3&	66.6&	55.2&	41.9&	30.8&	72.0&	49.9&	39.9&	34.6&	40.4&	36.7 \\ 
\cline{6-21}
                                     &               &               &               &              & \textbf{microwave} & \textbf{oven}          & \textbf{toaster}      & \textbf{sink}      & \textbf{refrigerator}  & \textbf{book}           & \textbf{clock}      & \textbf{vase}      & \textbf{scissors}      & \textbf{teddy-bear} & \textbf{hair-drier} & \textbf{toothbrush} & \textbf{\color{red}{person}}  & {\color{red}{\textbf{bike}}}   & \textbf{{\color{red}{car}}}      & \textbf{\color{red}{mbike}}       \\ 
\cline{6-21}
                                     &               &               &               &              & 31.9               & 35.6                   & 0.0                   & 28.0               & 42.3                   & 23.2                    & 48.5                & 36.7               & 38.6                   & 55.2                & 0.0                 & 0.0                 & 35.3             & 13.0            & 8.3               & 42.2                 \\
                                     &               &               &               &              & 32.2               & 36.6                   & 0.0                   & 27.6               & 44.2                   & 22.2                    & 51.3                & 37.5               & 44.7                   & 59.5                & 0.0                 & 0.0                 & 59.4             & 17.0            & 10.0              & 46.3                 \\
                                     &               &               &               &              & 34.7               & 50.1                   & 0.0                   & 37.6               & 56.7                   & 24.9                    & 58.3                & 38.1               & 45.0                   & 66.4                & 0.0                 & 29.2                & 67.4             & 43.8            & 17.5              & 57.5                 \\
                                     &               &               &               &              & 33.2               & 50.2                   & 0.0                   & 36.9               & 54.3                   & 24.5                    & 58.7                & 40.0               & 43.7                   & 67.2                & 0.0                 & 27.1                & 70.6             & 40.6            & 9.5               & 61.4                 \\ 
                                     &               &               &               &              & 50.3&	44.7&	3.3&	46.2&	66.4&	31.1&	61.0&	42.8&	46.6&	70.3&	0.0&	33.2&	65.7&	38.4&	25.7&	60.5 \\ 
\cline{6-21}
                                     &               &               &               &              & \textbf{\color{red}{aplane}}    & \textbf{\color{red}{bus}}           & \textbf{\color{red}{train}}        & \textbf{\color{red}{boat}}      & \textbf{\color{red}{bird}}          & \textbf{\color{red}{cat}}            & \textbf{\color{red}{dog}}        & \textbf{\color{red}{horse}}     & \textbf{\color{red}{sheep}}         & \textbf{\color{red}{cow}}        & \textbf{\color{red}{bott}}       & \textbf{\color{red}{chair}}      & \textbf{\color{red}{sofa}}    & \textbf{\color{red}{plant}}  & \textbf{\color{red}{d.table}}  & \textbf{\color{red}{tv}}          \\ 
\cline{6-21}
                                     &               &               &               &              & 12.1               & 15.5                   & 22.9                  & 15.8               & 18.4                   & 37.0                    & 23.0                & 31.9               & 28.6                   & 20.4                & 11.8                & 14.4                & 12.8             & 11.3            & 13.6              & 18.3                 \\
                                     &               &               &               &              & 23.8               & 7.4                    & 19.1                  & 13.1               & 43.9                   & 55.0                    & 41.3                & 49.6               & 39.9                   & 41.2                & 12.4                & 14.9                & 16.8             & 10.2            & 18.2              & 23.5                 \\
                                     &               &               &               &              & 45.7               & 31.9                   & 47.4                  & 27.0               & 41.5                   & 56.0                    & 52.3                & 62.1               & 39.3                   & 48.7                & 20.0                & 13.7                & 17.3             & 12.7            & 11.2              & 24.5                 \\
                                     &               &               &               &              & 52.6               & 27.3                   & 55.7                  & 36.3               & 44.0                   & 57.9                    & 51.4                & 61.3               & 51.1                   & 48.5                & 20.3                & 14.7                & 13.6             & 13.8            & 13.5              & 24.2                 \\ 
                                     &               &               &               &              & 57.8&	26.6&	43.9&	32.9&	51.0&	66.1&	54.9&	64.4&	61.0&	53.5&	25.4&	17.3&	18.9&	14.6&	8.6&	32.5         
\end{tabular}
\end{adjustbox}
\caption{Per class results on COCO for the COCO-to-VOC setting, expressed in mIoU. Best method in bold. VOC classes in red.} 
\label{tab:coco2voc-coco}
\end{table*}
